# Supplementary material for: On the accuracy of a recent regularized nuclear potential
Source: arXiv:2302.09557 ancillary file (2023-05-20)
Supplement: Supplementary file 1 [file si.pdf]

# Supporting Information:

## On the accuracy of a recent regularized nuclear potential

Susi Lehtola<sup>\*,†</sup>

*Department of Chemistry, University of Helsinki, P.O. Box 55, FI-00014 University of Helsinki, Finland*

E-mail: susi.lehtola@alumni.helsinki.fi

First, we show the full set of regularization errors in atomic total energies. Positive energy differences ( $E^{\text{regularized}} > E^{\text{Coulomb}}$ ) are shown with blue squares and negative energy differences ( $E^{\text{regularized}} < E^{\text{Coulomb}}$ ) with red triangles in all figures.

- He atom: HF in fig. S1, PW92 in fig. S2, PBE in fig. S3, TASKCC in fig. S4.
- Be atom: HF in fig. S5, PW92 in fig. S6, PBE in fig. S7, TASKCC in fig. S8.
- Ne atom: HF in fig. S9, PW92 in fig. S10, PBE in fig. S11, TASKCC in fig. S12.
- Mg atom: HF in fig. S13, PW92 in fig. S14, PBE in fig. S15, TASKCC in fig. S16.
- Ar atom: HF in fig. S17, PW92 in fig. S18, PBE in fig. S19, TASKCC in fig. S20.
- Ca atom: HF in fig. S21, PW92 in fig. S22, PBE in fig. S23, TASKCC in fig. S24.
- Zn atom: HF in fig. S25, PW92 in fig. S26, PBE in fig. S27, TASKCC in fig. S28.
- Kr atom: HF in fig. S29, PW92 in fig. S30, PBE in fig. S31, TASKCC in fig. S32.
- Sr atom: HF in fig. S33, PW92 in fig. S34, PBE in fig. S35, TASKCC in fig. S36.
- Cd atom: HF in fig. S37, PW92 in fig. S38, PBE in fig. S39, TASKCC in fig. S40.
- Xe atom: HF in fig. S41, PW92 in fig. S42, PBE in fig. S43, TASKCC in fig. S44.

Then, we also show the regularization errors in orbital energies and positions of orbital density maxima for all calculations:

- He atom: HF in tables S1 and S2, respectively, PW92 in tables S3 and S4, respectively, PBE in tables S5 and S6, respectively, TASKCC in tables S7 and S8, respectively.
- Be atom: HF in tables S9 and S10, respectively, PW92 in tables S11 and S12, respectively, PBE in tables S13 and S14, respectively, TASKCC in tables S15 and S16, respectively.
- Ne atom: HF in tables S17 and S18, respectively, PW92 in tables S19 and S20, respectively, PBE in tables S21 and S22, respectively, TASKCC in tables S23 and S24, respectively.
- Mg atom: HF in tables S25 and S26, respectively, PW92 in tables S27 and S28, respectively, PBE in tables S29 and S30, respectively, TASKCC in tables S31 and S32, respectively.

- Ar atom: HF in tables S33 and S34, respectively, PW92 in tables S35 and S36, respectively, PBE in tables S37 and S38, respectively, TASKCC in tables S39 and S40, respectively.
- Ca atom: HF in tables S41 and S42, respectively, PW92 in tables S43 and S44, respectively, PBE in tables S45 and S46, respectively, TASKCC in tables S47 and S48, respectively.
- Zn atom: HF in tables S49 and S50, respectively, PW92 in tables S51 and S52, respectively, PBE in tables S53 and S54, respectively, TASKCC in tables S55 and S56, respectively.
- Kr atom: HF in tables S57 and S58, respectively, PW92 in tables S59 and S60, respectively, PBE in tables S61 and S62, respectively, TASKCC in tables S63 and S64, respectively.
- Sr atom: HF in tables S65 and S66, respectively, PW92 in tables S67 and S68, respectively, PBE in tables S69 and S70, respectively, TASKCC in tables S71 and S72, respectively.
- Cd atom: HF in tables S73 and S74, respectively, PW92 in tables S75 and S76, respectively, PBE in tables S77 and S78, respectively, TASKCC in tables S79 and S80, respectively.
- Xe atom: HF in tables S81 and S82, respectively, PW92 in tables S83 and S84, respectively, PBE in tables S85 and S86, respectively, TASKCC in tables S87 and S88, respectively.

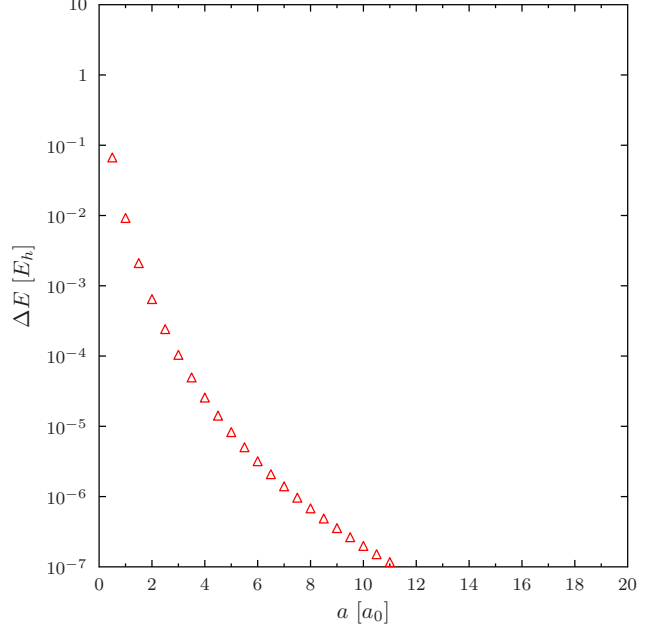

Figure S1: Regularization error in the total energy of the He atom calculated with HF.

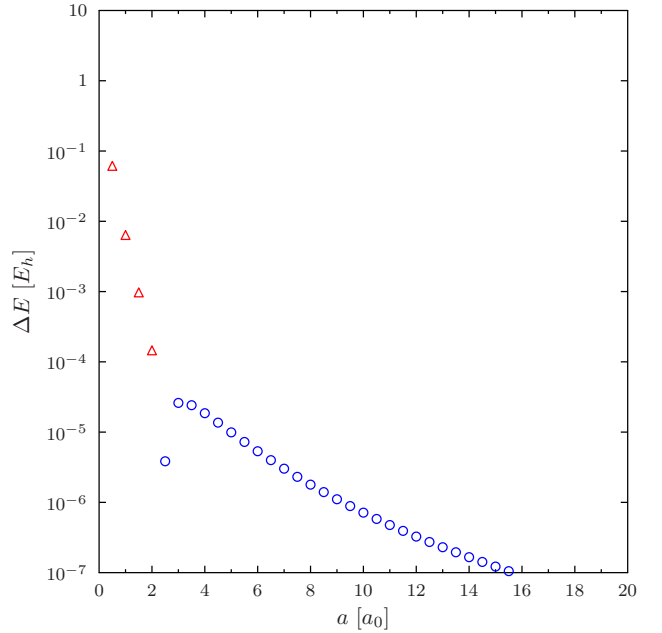

Figure S2: Regularization error in the total energy of the He atom calculated with PW92.

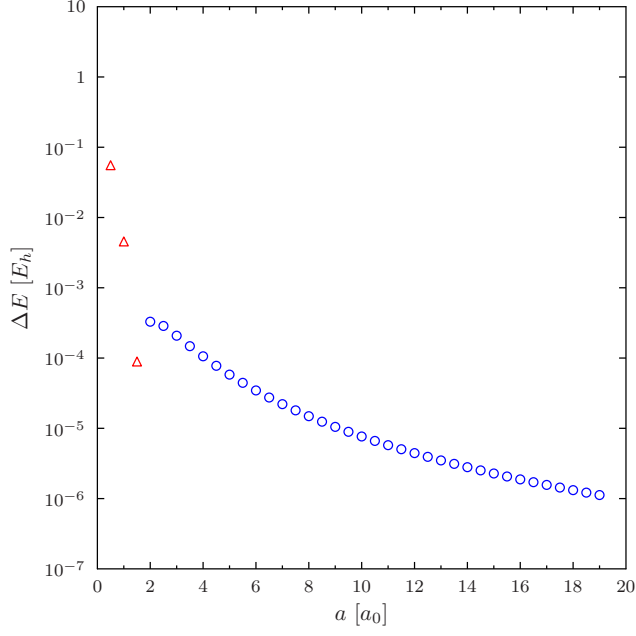

Figure S3: Regularization error in the total energy of the He atom calculated with PBE.

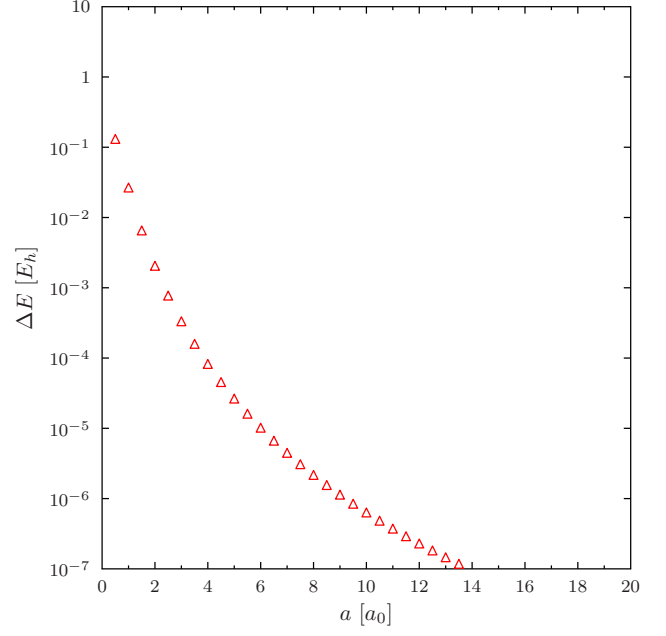

Figure S5: Regularization error in the total energy of the Be atom calculated with HF.

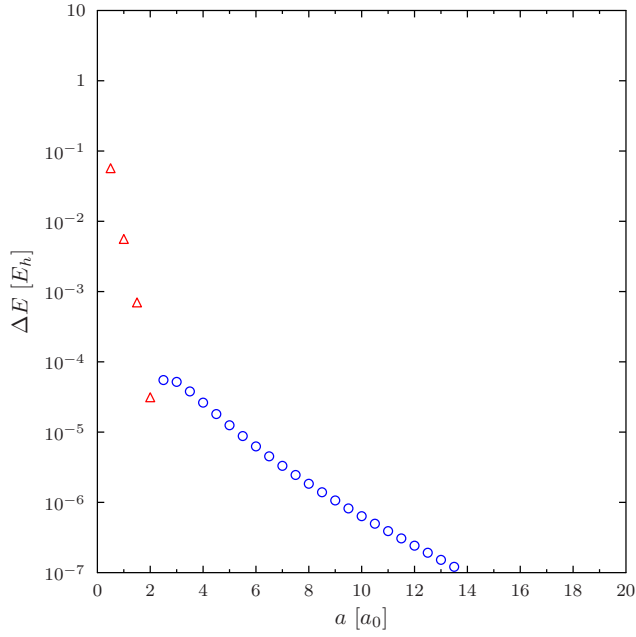

Figure S4: Regularization error in the total energy of the He atom calculated with TASKCC.

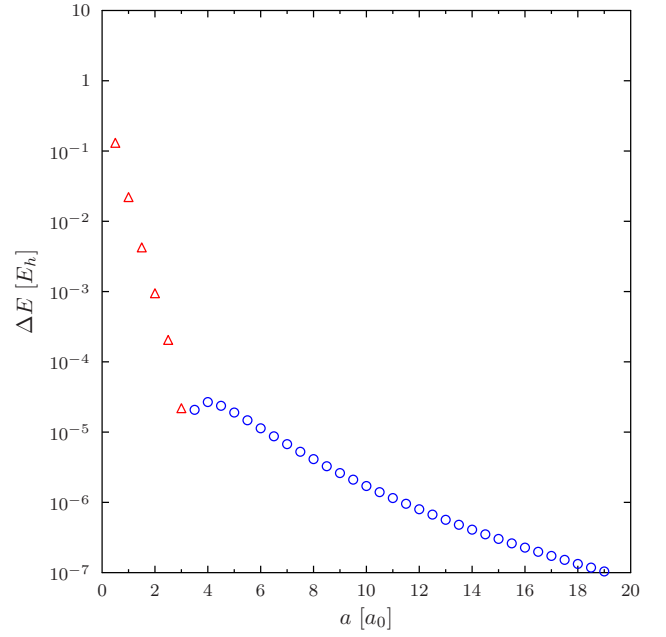

Figure S6: Regularization error in the total energy of the Be atom calculated with PW92.

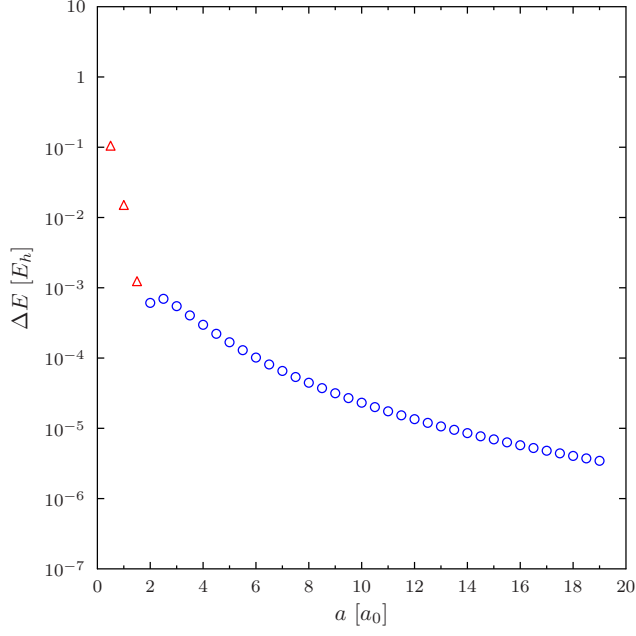

Figure S7: Regularization error in the total energy of the Be atom calculated with PBE.

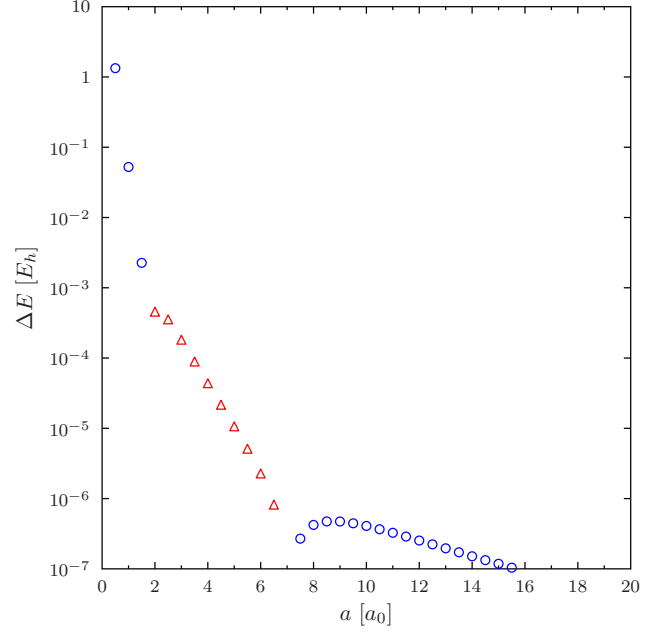

Figure S9: Regularization error in the total energy of the Ne atom calculated with HF.

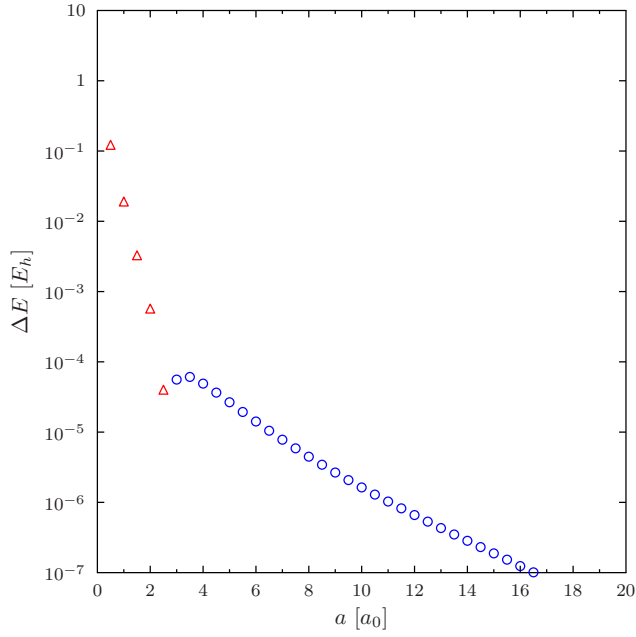

Figure S8: Regularization error in the total energy of the Be atom calculated with TASKCC.

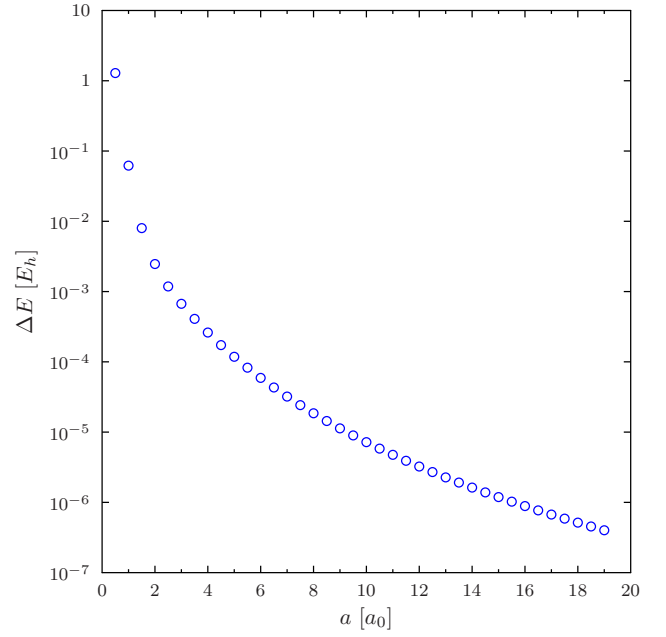

Figure S10: Regularization error in the total energy of the Ne atom calculated with PW92.

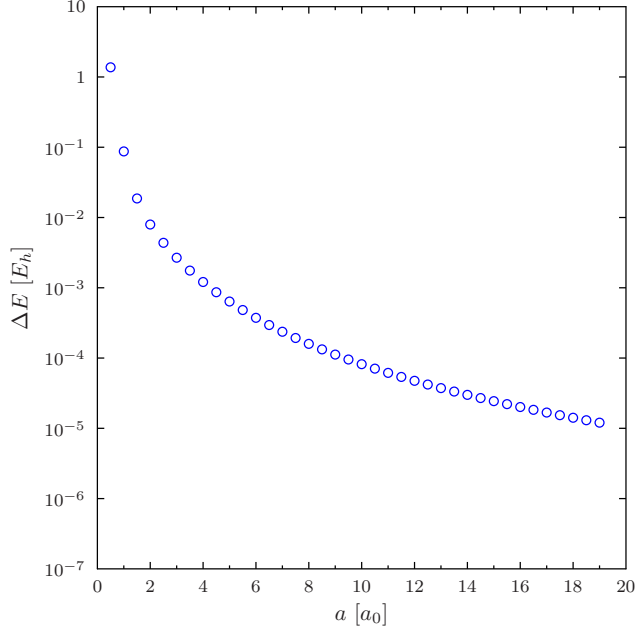

Figure S11: Regularization error in the total energy of the Ne atom calculated with PBE.

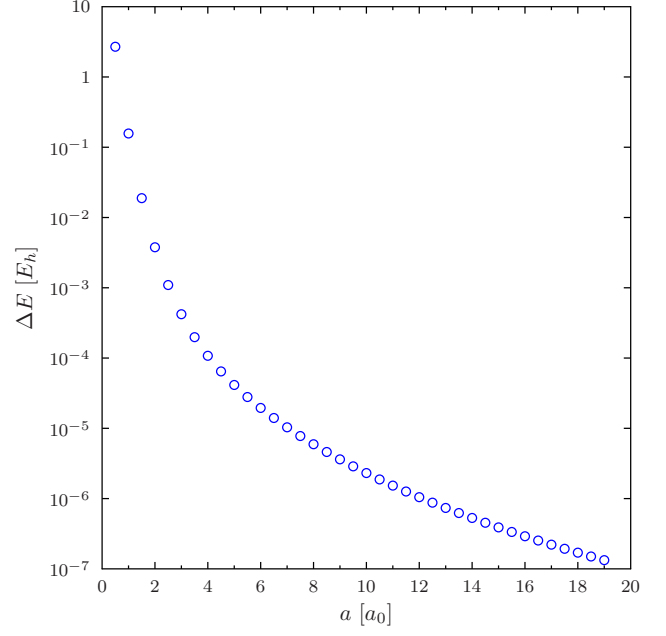

Figure S13: Regularization error in the total energy of the Mg atom calculated with HF.

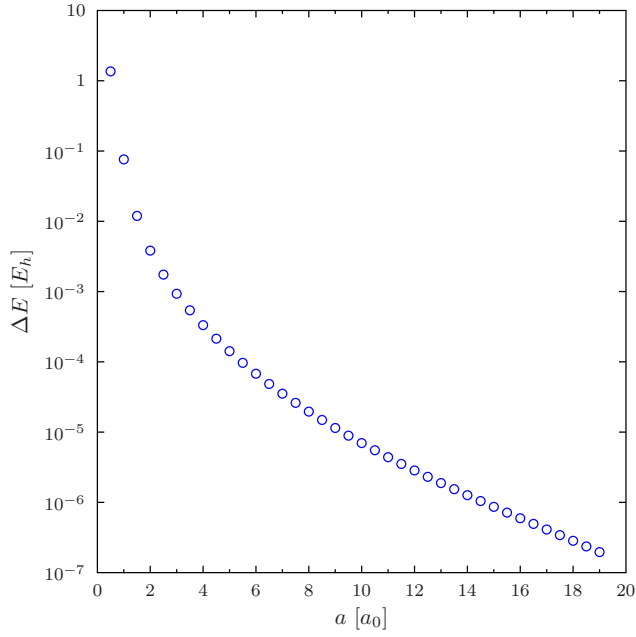

Figure S12: Regularization error in the total energy of the Ne atom calculated with TASKCC.

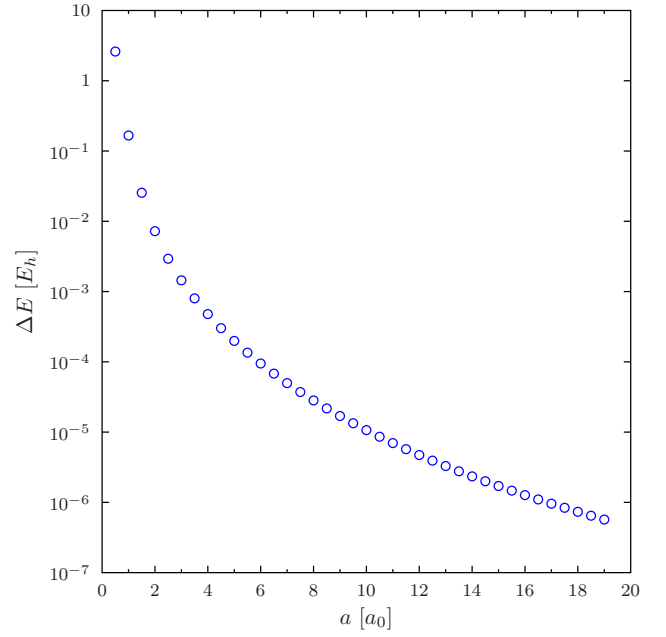

Figure S14: Regularization error in the total energy of the Mg atom calculated with PW92.

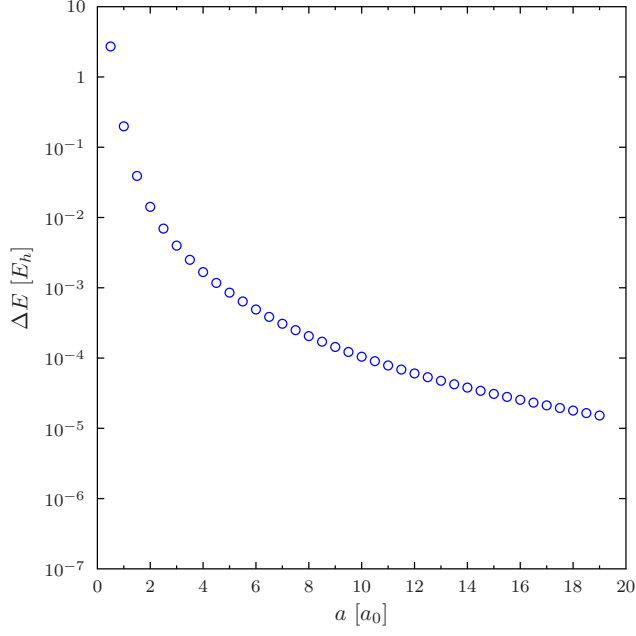

Figure S15: Regularization error in the total energy of the Mg atom calculated with PBE.

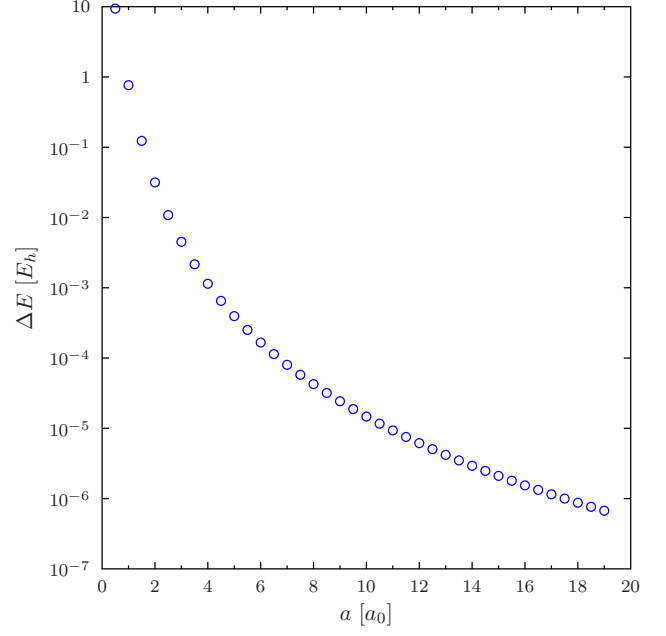

Figure S17: Regularization error in the total energy of the Ar atom calculated with HF.

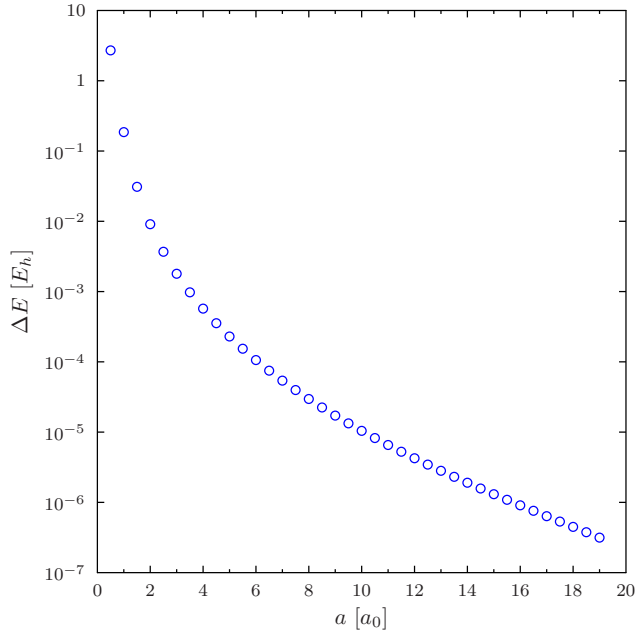

Figure S16: Regularization error in the total energy of the Mg atom calculated with TASKCC.

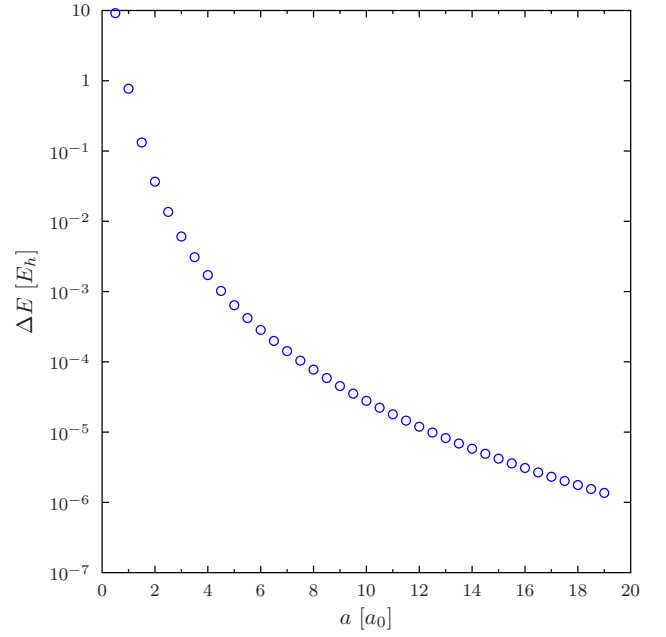

Figure S18: Regularization error in the total energy of the Ar atom calculated with PW92.

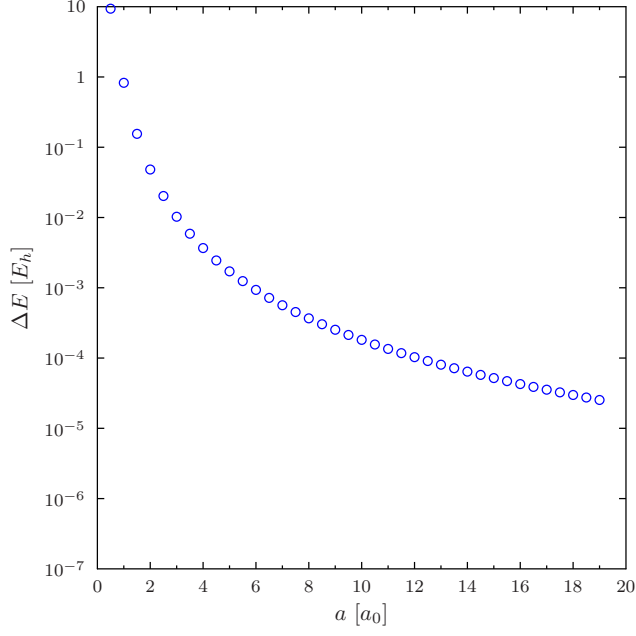

Figure S19: Regularization error in the total energy of the Ar atom calculated with PBE.

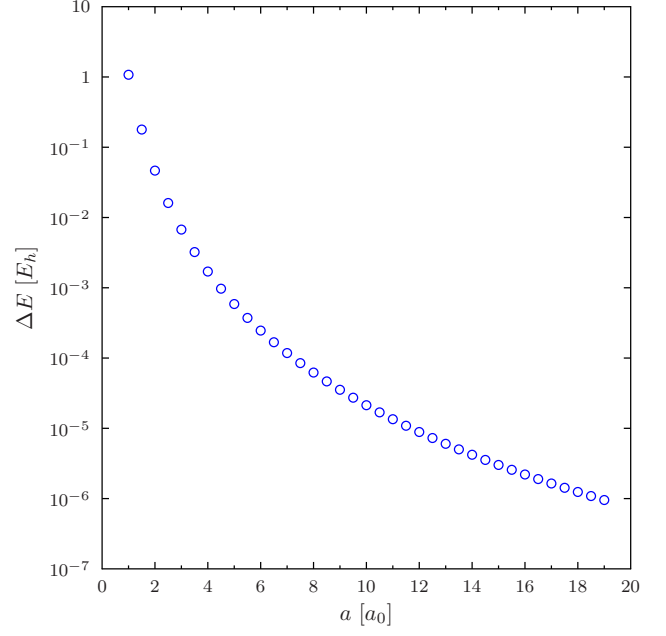

Figure S21: Regularization error in the total energy of the Ca atom calculated with HF.

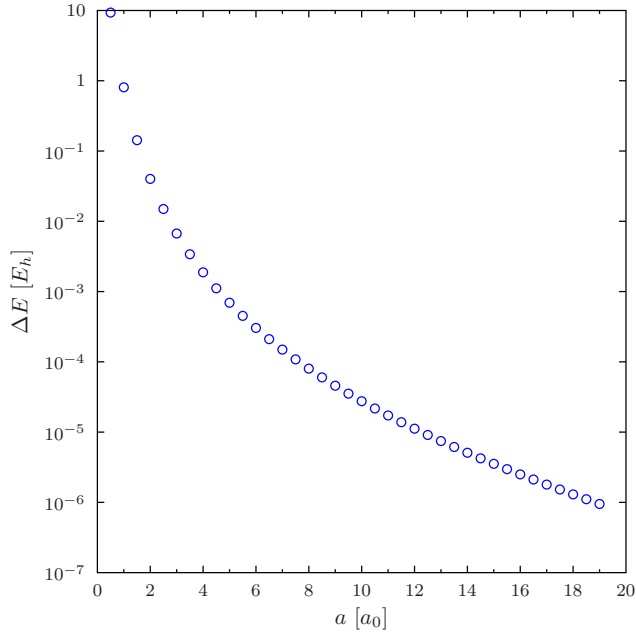

Figure S20: Regularization error in the total energy of the Ar atom calculated with TASKCC.

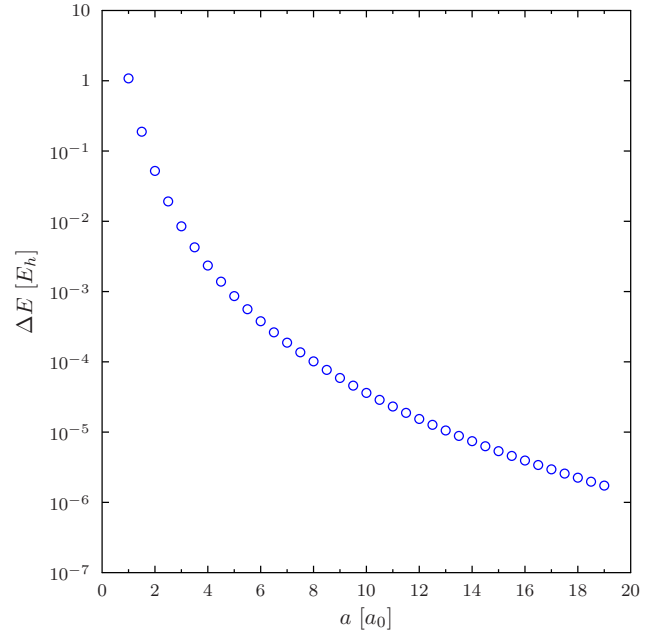

Figure S22: Regularization error in the total energy of the Ca atom calculated with PW92.

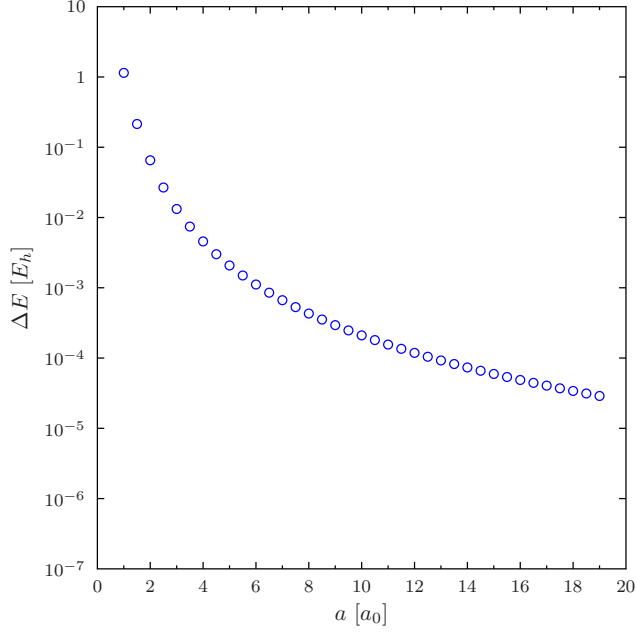

Figure S23: Regularization error in the total energy of the Ca atom calculated with PBE.

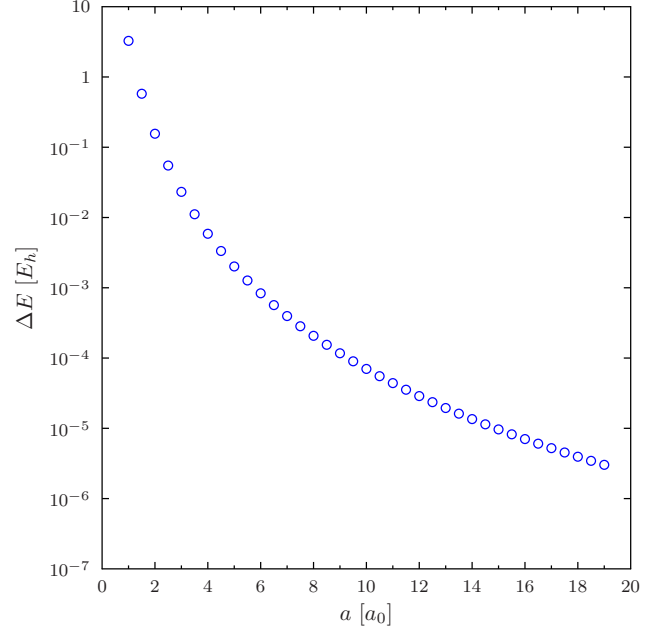

Figure S25: Regularization error in the total energy of the Zn atom calculated with HF.

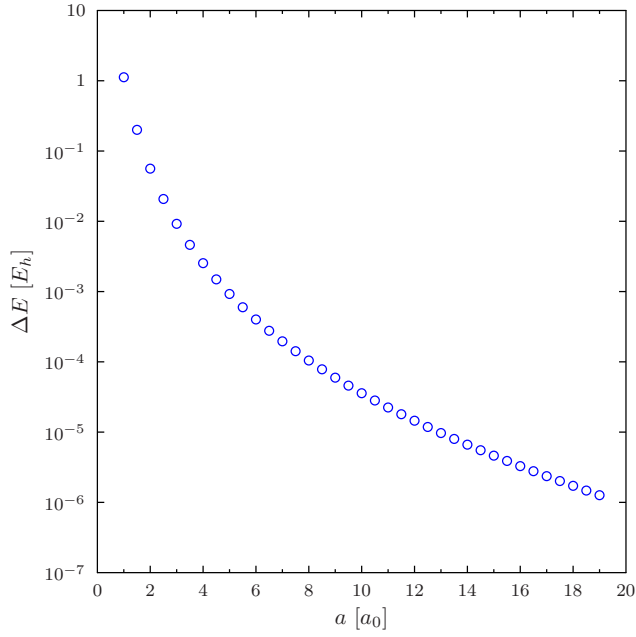

Figure S24: Regularization error in the total energy of the Ca atom calculated with TASKCC.

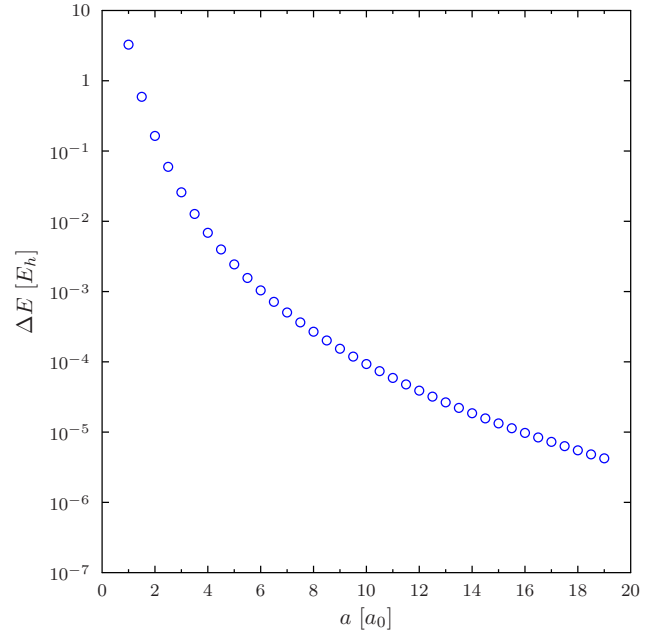

Figure S26: Regularization error in the total energy of the Zn atom calculated with PW92.



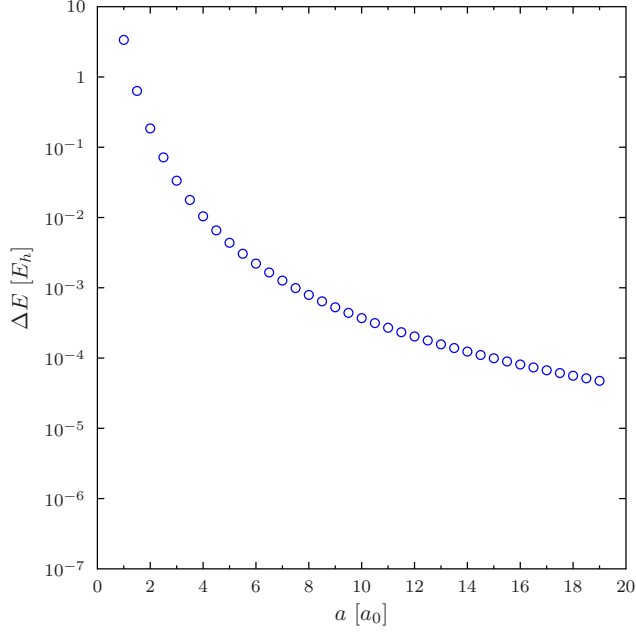

Figure S27: Regularization error in the total energy of the Zn atom calculated with PBE.

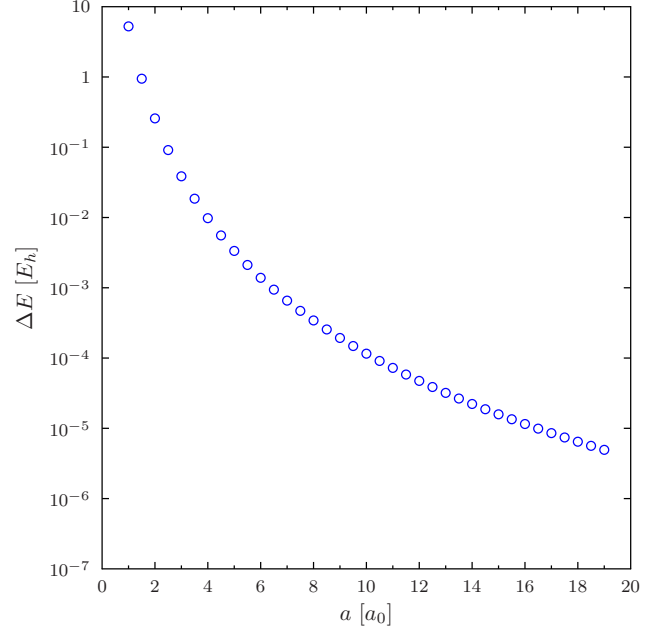

Figure S29: Regularization error in the total energy of the Kr atom calculated with HF.

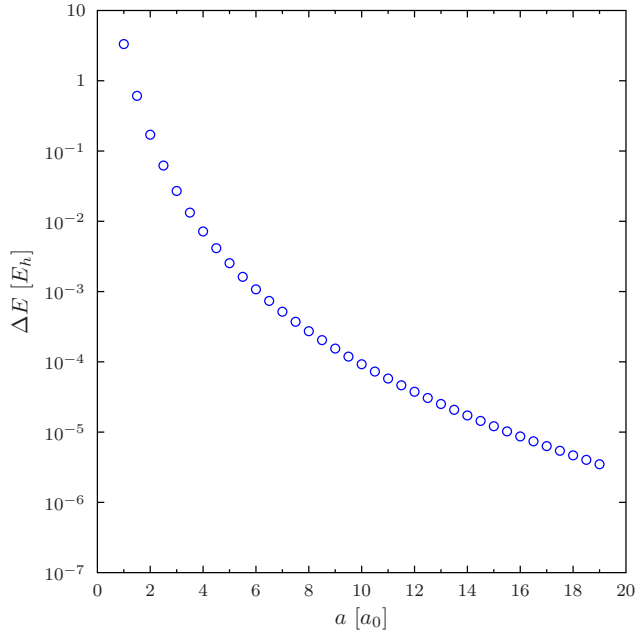

Figure S28: Regularization error in the total energy of the Zn atom calculated with TASKCC.

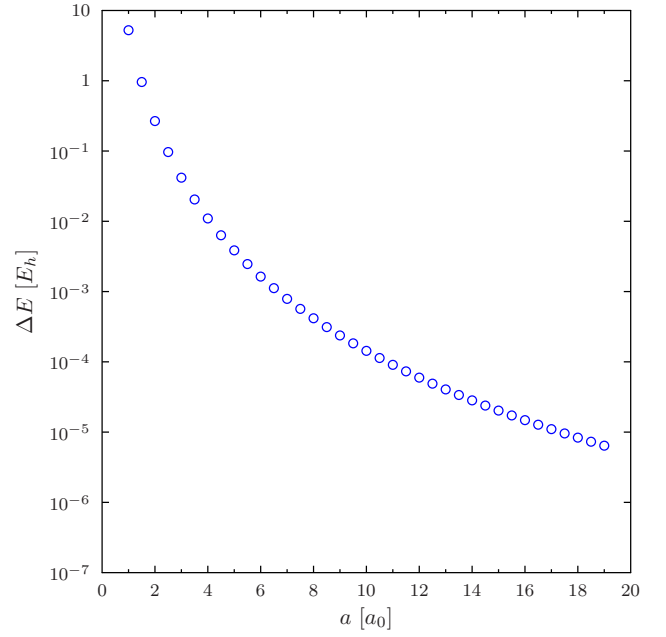

Figure S30: Regularization error in the total energy of the Kr atom calculated with PW92.

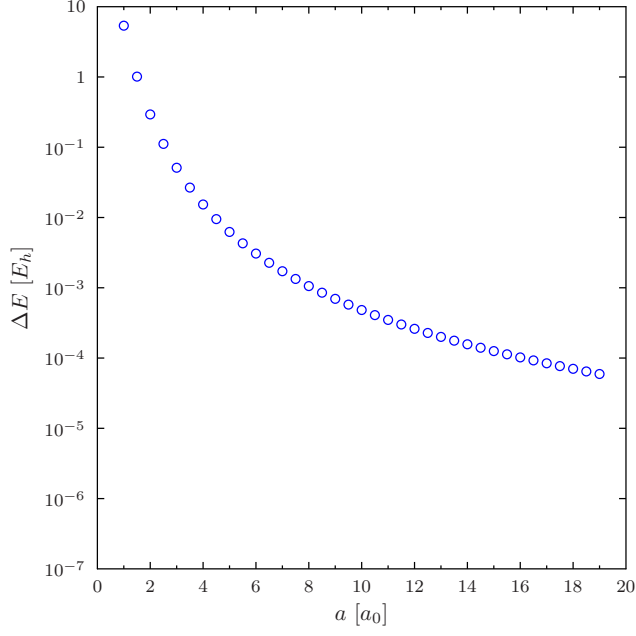

Figure S31: Regularization error in the total energy of the Kr atom calculated with PBE.

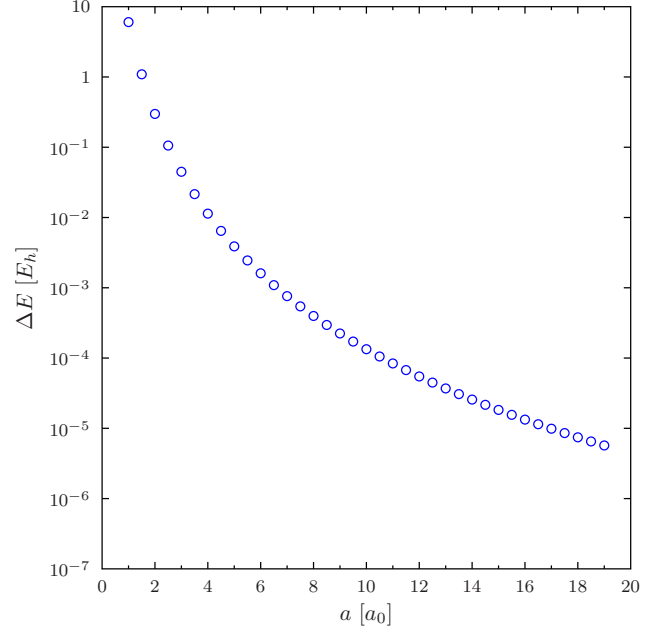

Figure S33: Regularization error in the total energy of the Sr atom calculated with HF.

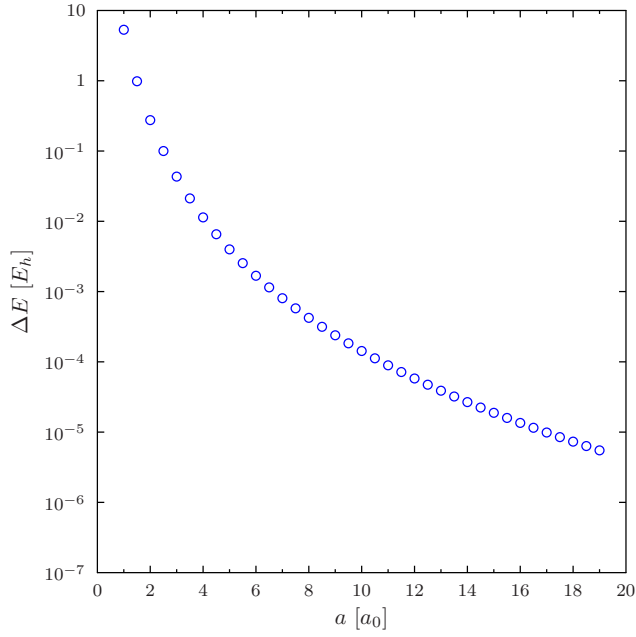

Figure S32: Regularization error in the total energy of the Kr atom calculated with TASKCC.

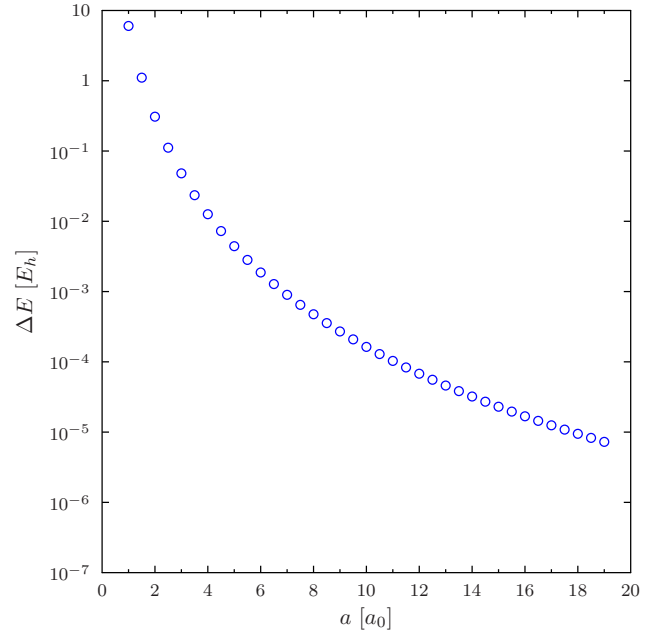

Figure S34: Regularization error in the total energy of the Sr atom calculated with PW92.

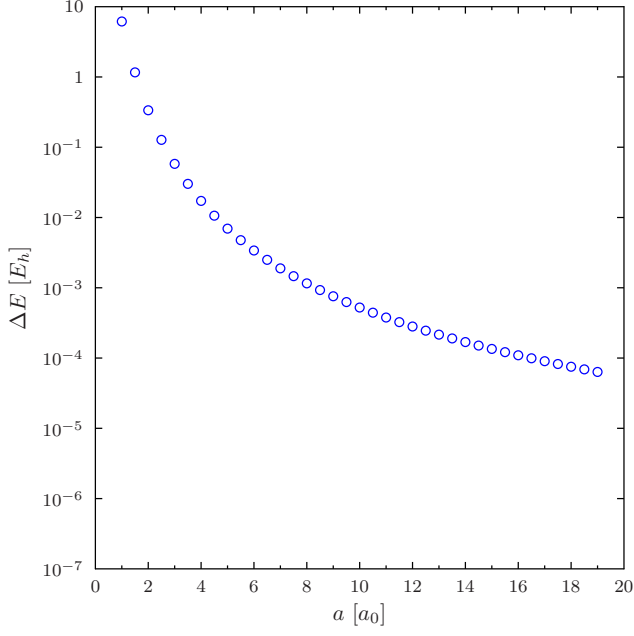

Figure S35: Regularization error in the total energy of the Sr atom calculated with PBE.

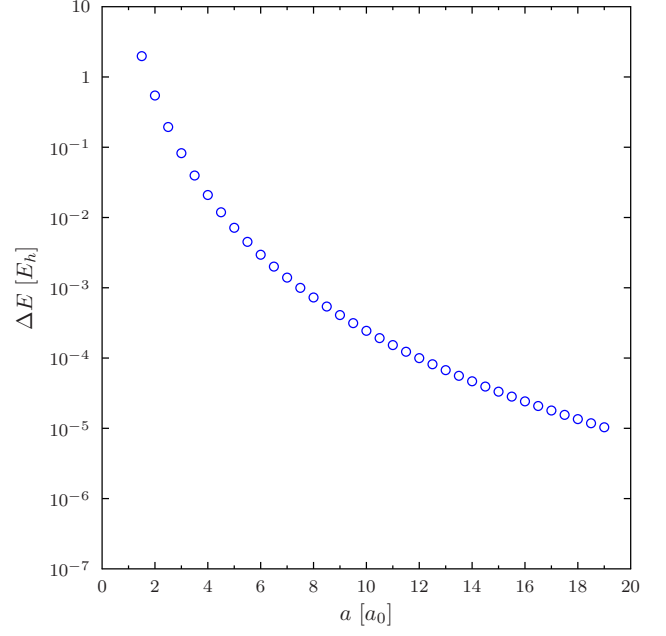

Figure S37: Regularization error in the total energy of the Cd atom calculated with HF.

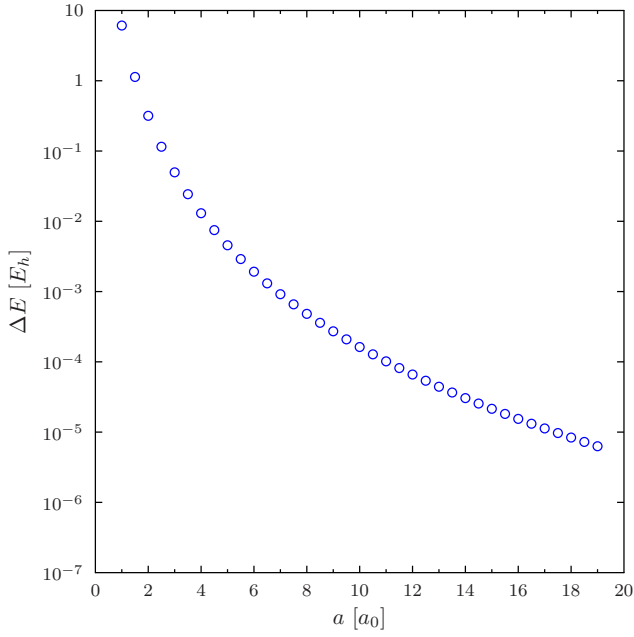

Figure S36: Regularization error in the total energy of the Sr atom calculated with TASKCC.

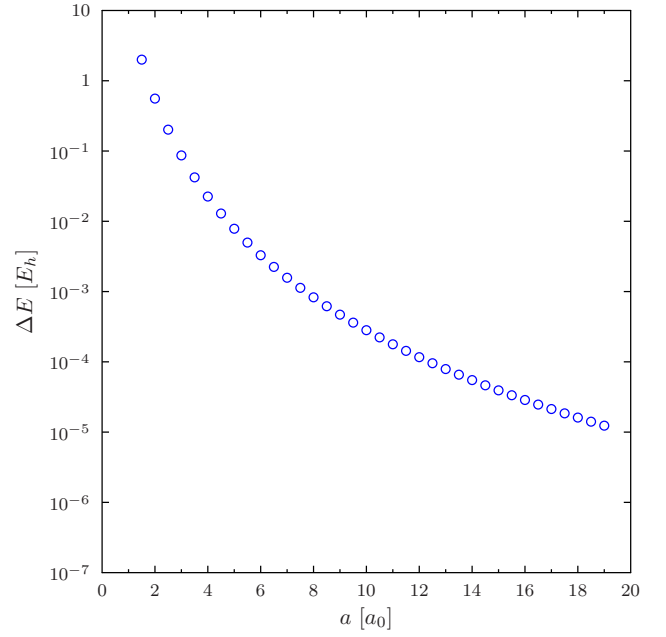

Figure S38: Regularization error in the total energy of the Cd atom calculated with PW92.

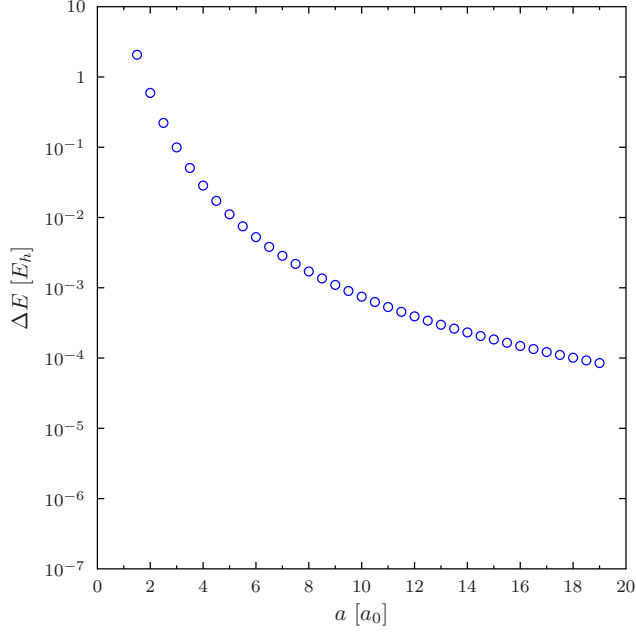

Figure S39: Regularization error in the total energy of the Cd atom calculated with PBE.

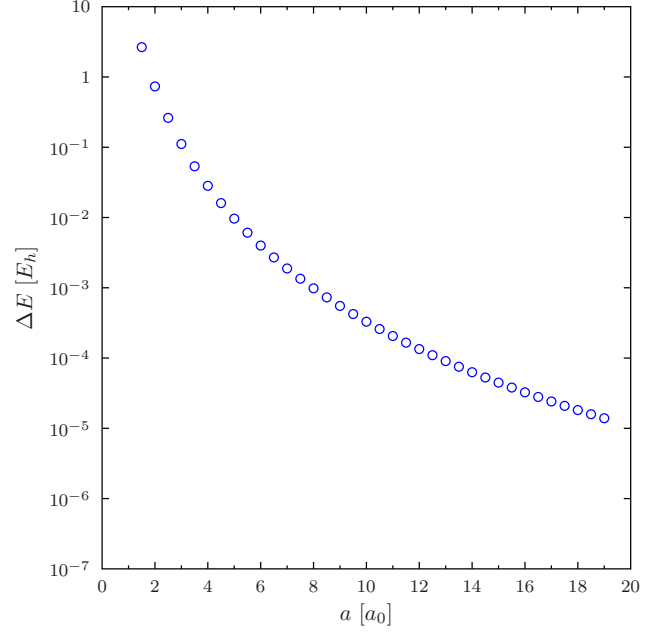

Figure S41: Regularization error in the total energy of the Xe atom calculated with HF.

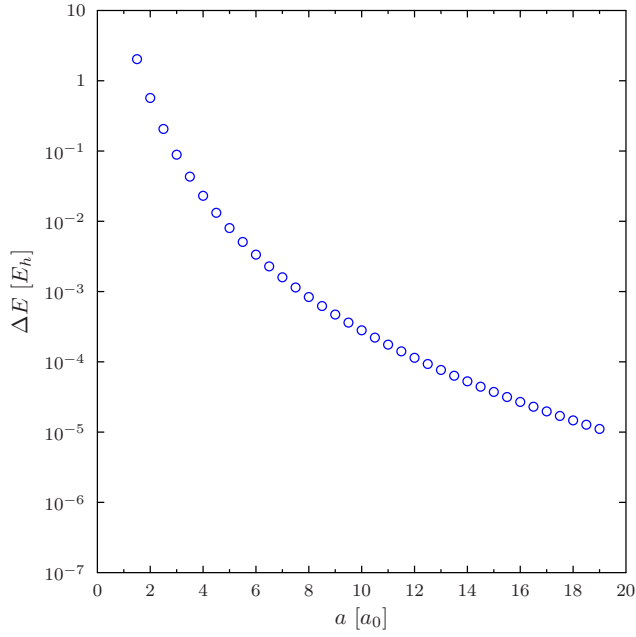

Figure S40: Regularization error in the total energy of the Cd atom calculated with TASKCC.

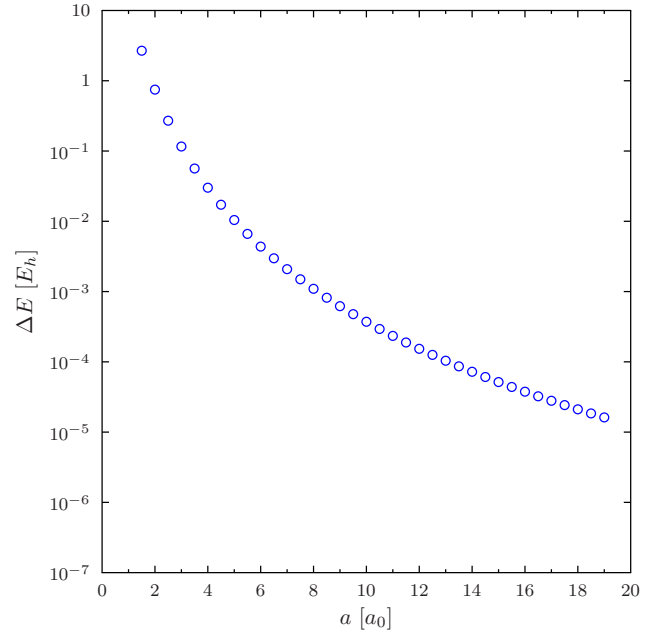

Figure S42: Regularization error in the total energy of the Xe atom calculated with PW92.

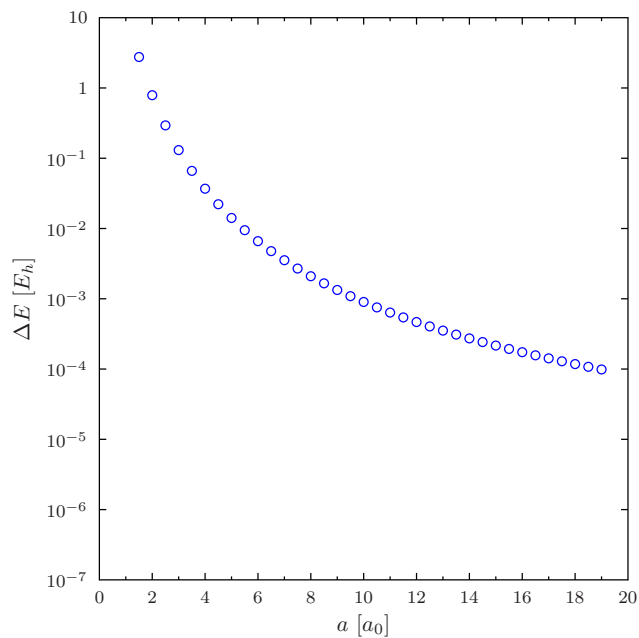

Figure S43: Regularization error in the total energy of the Xe atom calculated with PBE.

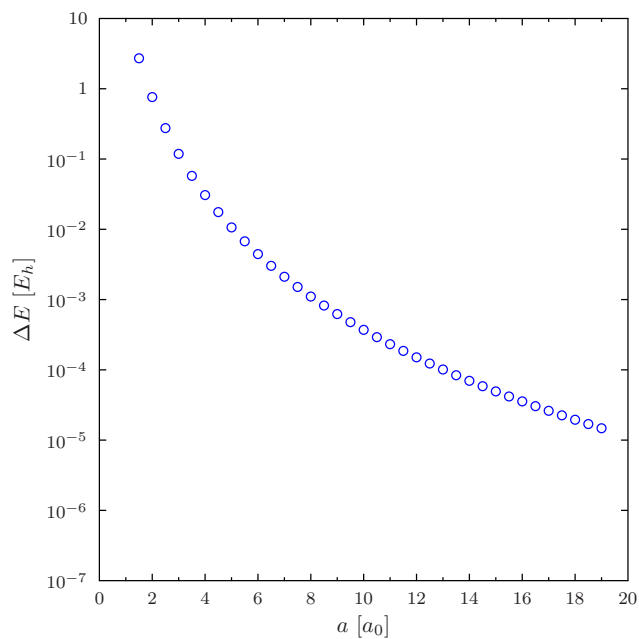

Figure S44: Regularization error in the total energy of the Xe atom calculated with TASKCC.

Table S1: Errors in orbital energies in  $E_h$  for the He atom computed with HF and the regularized potential with various values of  $a$ . The values obtained with the Coulomb potential of the point nucleus are shown in the last column. For comparison, the last row shows the errors in total energy  $\Delta E$  from the point nucleus value shown in the last column.

| Energy     | $a = 1.0$  | $a = 2.0$  | $a = 3.0$  | $a = 5.0$  | $a = 7.0$  | point nucleus |
|------------|------------|------------|------------|------------|------------|---------------|
| 1s         | -0.0052    | -0.0003    | -0.0001    | -0.0000    | -0.0000    | -0.9180       |
| $\Delta E$ | -0.0088312 | -0.0006190 | -0.0000995 | -0.0000079 | -0.0000013 | -2.8616800    |

Table S2: Errors in positions of orbital density maxima in bohr for the He atom computed with HF and the regularized potential with various values of  $a$ . The values obtained with the Coulomb potential of the point nucleus are shown in the last column.

| Energy | $a = 1.0$ | $a = 2.0$ | $a = 3.0$ | $a = 5.0$ | $a = 7.0$ | point nucleus |
|--------|-----------|-----------|-----------|-----------|-----------|---------------|
| 1s     | -0.016784 | -0.002700 | -0.000052 | -0.000004 | -0.000000 | 0.569145      |

Table S3: Errors in orbital energies in  $E_h$  for the He atom computed with PW92 and the regularized potential with various values of  $a$ . The values obtained with the Coulomb potential of the point nucleus are shown in the last column. For comparison, the last row shows the errors in total energy  $\Delta E$  from the point nucleus value shown in the last column.

| Energy     | $a = 1.0$  | $a = 2.0$  | $a = 3.0$ | $a = 5.0$ | $a = 7.0$ | point nucleus |
|------------|------------|------------|-----------|-----------|-----------|---------------|
| 1s         | -0.0036    | -0.0002    | -0.0000   | 0.0000    | 0.0000    | -0.5703       |
| $\Delta E$ | -0.0061111 | -0.0001397 | 0.0000260 | 0.0000099 | 0.0000030 | -2.8344552    |

Table S4: Errors in positions of orbital density maxima in bohr for the He atom computed with PW92 and the regularized potential with various values of  $a$ . The values obtained with the Coulomb potential of the point nucleus are shown in the last column.

| Energy | $a = 1.0$ | $a = 2.0$ | $a = 3.0$ | $a = 5.0$ | $a = 7.0$ | point nucleus |
|--------|-----------|-----------|-----------|-----------|-----------|---------------|
| 1s     | -0.016881 | -0.002732 | -0.000032 | 0.000001  | 0.000001  | 0.569641      |

Table S5: Errors in orbital energies in  $E_h$  for the He atom computed with PBE and the regularized potential with various values of  $a$ . The values obtained with the Coulomb potential of the point nucleus are shown in the last column. For comparison, the last row shows the errors in total energy  $\Delta E$  from the point nucleus value shown in the last column.

| Energy     | $a = 1.0$  | $a = 2.0$ | $a = 3.0$ | $a = 5.0$ | $a = 7.0$ | point nucleus |
|------------|------------|-----------|-----------|-----------|-----------|---------------|
| 1s         | -0.0040    | -0.0001   | -0.0000   | 0.0000    | 0.0000    | -0.5793       |
| $\Delta E$ | -0.0043708 | 0.0003289 | 0.0002079 | 0.0000581 | 0.0000221 | -2.8929349    |

Table S6: Errors in positions of orbital density maxima in bohr for the He atom computed with PBE and the regularized potential with various values of  $a$ . The values obtained with the Coulomb potential of the point nucleus are shown in the last column.

| Energy | $a = 1.0$ | $a = 2.0$ | $a = 3.0$ | $a = 5.0$ | $a = 7.0$ | point nucleus |
|--------|-----------|-----------|-----------|-----------|-----------|---------------|
| 1s     | -0.014547 | -0.003028 | -0.000016 | 0.000006  | 0.000003  | 0.560260      |

Table S7: Errors in orbital energies in  $E_h$  for the He atom computed with TASKCC and the regularized potential with various values of  $a$ . The values obtained with the Coulomb potential of the point nucleus are shown in the last column. For comparison, the last row shows the errors in total energy  $\Delta E$  from the point nucleus value shown in the last column.

| Energy     | $a = 1.0$  | $a = 2.0$  | $a = 3.0$ | $a = 5.0$ | $a = 7.0$ | point nucleus |
|------------|------------|------------|-----------|-----------|-----------|---------------|
| 1s         | -0.0042    | -0.0002    | -0.0000   | 0.0000    | 0.0000    | -0.6426       |
| $\Delta E$ | -0.0053662 | -0.0000300 | 0.0000518 | 0.0000125 | 0.0000033 | -2.9794485    |

Table S8: Errors in positions of orbital density maxima in bohr for the He atom computed with TASKCC and the regularized potential with various values of  $a$ . The values obtained with the Coulomb potential of the point nucleus are shown in the last column.

| Energy | $a = 1.0$ | $a = 2.0$ | $a = 3.0$ | $a = 5.0$ | $a = 7.0$ | point nucleus |
|--------|-----------|-----------|-----------|-----------|-----------|---------------|
| 1s     | -0.013521 | -0.002950 | -0.000027 | 0.000002  | 0.000001  | 0.559246      |

Table S9: Errors in orbital energies in  $E_h$  for the Be atom computed with HF and the regularized potential with various values of  $a$ . The values obtained with the Coulomb potential of the point nucleus are shown in the last column. For comparison, the last row shows the errors in total energy  $\Delta E$  from the point nucleus value shown in the last column.

| Energy     | $a = 1.0$  | $a = 2.0$  | $a = 3.0$  | $a = 5.0$  | $a = 7.0$  | point nucleus |
|------------|------------|------------|------------|------------|------------|---------------|
| 1s         | -0.0236    | -0.0015    | -0.0002    | -0.0000    | -0.0000    | -4.7327       |
| 2s         | 0.0001     | -0.0000    | -0.0000    | -0.0000    | -0.0000    | -0.3093       |
| $\Delta E$ | -0.0255920 | -0.0019684 | -0.0003195 | -0.0000254 | -0.0000043 | -14.5730232   |

Table S10: Errors in positions of orbital density maxima in bohr for the Be atom computed with HF and the regularized potential with various values of  $a$ . The values obtained with the Coulomb potential of the point nucleus are shown in the last column.

| Energy | $a = 1.0$ | $a = 2.0$ | $a = 3.0$ | $a = 5.0$ | $a = 7.0$ | point nucleus |
|--------|-----------|-----------|-----------|-----------|-----------|---------------|
| 1s     | -0.003048 | -0.001723 | -0.000024 | -0.000001 | -0.000000 | 0.267051      |
| 2s     | 0.000854  | -0.000197 | -0.000038 | -0.000003 | 0.000000  | 2.050591      |

Table S11: Errors in orbital energies in  $E_h$  for the Be atom computed with PW92 and the regularized potential with various values of  $a$ . The values obtained with the Coulomb potential of the point nucleus are shown in the last column. For comparison, the last row shows the errors in total energy  $\Delta E$  from the point nucleus value shown in the last column.

| Energy     | $a = 1.0$  | $a = 2.0$  | $a = 3.0$  | $a = 5.0$ | $a = 7.0$ | point nucleus |
|------------|------------|------------|------------|-----------|-----------|---------------|
| 1s         | -0.0255    | -0.0013    | -0.0001    | -0.0000   | 0.0000    | -3.8561       |
| 2s         | -0.0000    | -0.0000    | -0.0000    | -0.0000   | 0.0000    | -0.2058       |
| $\Delta E$ | -0.0211475 | -0.0009060 | -0.0000210 | 0.0000190 | 0.0000067 | -14.4464735   |

Table S12: Errors in positions of orbital density maxima in bohr for the Be atom computed with PW92 and the regularized potential with various values of  $a$ . The values obtained with the Coulomb potential of the point nucleus are shown in the last column.

| Energy | $a = 1.0$ | $a = 2.0$ | $a = 3.0$ | $a = 5.0$ | $a = 7.0$ | point nucleus |
|--------|-----------|-----------|-----------|-----------|-----------|---------------|
| 1s     | -0.003532 | -0.001701 | -0.000020 | -0.000000 | 0.000000  | 0.268766      |
| 2s     | 0.000747  | -0.000150 | -0.000020 | 0.000000  | 0.000000  | 2.041544      |

Table S13: Errors in orbital energies in  $E_h$  for the Be atom computed with PBE and the regularized potential with various values of  $a$ . The values obtained with the Coulomb potential of the point nucleus are shown in the last column. For comparison, the last row shows the errors in total energy  $\Delta E$  from the point nucleus value shown in the last column.

| Energy     | $a = 1.0$  | $a = 2.0$ | $a = 3.0$ | $a = 5.0$ | $a = 7.0$ | point nucleus |
|------------|------------|-----------|-----------|-----------|-----------|---------------|
| 1s         | -0.0259    | -0.0011   | -0.0001   | 0.0000    | 0.0000    | -3.9026       |
| 2s         | 0.0000     | -0.0000   | -0.0000   | 0.0000    | 0.0000    | -0.2061       |
| $\Delta E$ | -0.0144345 | 0.0006093 | 0.0005475 | 0.0001677 | 0.0000655 | -14.6299477   |

Table S14: Errors in positions of orbital density maxima in bohr for the Be atom computed with PBE and the regularized potential with various values of  $a$ . The values obtained with the Coulomb potential of the point nucleus are shown in the last column.

| Energy | $a = 1.0$ | $a = 2.0$ | $a = 3.0$ | $a = 5.0$ | $a = 7.0$ | point nucleus |
|--------|-----------|-----------|-----------|-----------|-----------|---------------|
| 1s     | -0.002851 | -0.001780 | -0.000015 | 0.000002  | 0.000001  | 0.266176      |
| 2s     | 0.001050  | -0.000090 | 0.000003  | 0.000006  | 0.000002  | 2.042185      |

Table S15: Errors in orbital energies in  $E_h$  for the Be atom computed with TASKCC and the regularized potential with various values of  $a$ . The values obtained with the Coulomb potential of the point nucleus are shown in the last column. For comparison, the last row shows the errors in total energy  $\Delta E$  from the point nucleus value shown in the last column.

| Energy     | $a = 1.0$  | $a = 2.0$  | $a = 3.0$ | $a = 5.0$ | $a = 7.0$ | point nucleus |
|------------|------------|------------|-----------|-----------|-----------|---------------|
| 1s         | -0.0249    | -0.0012    | -0.0001   | 0.0000    | 0.0000    | -4.0563       |
| 2s         | -0.0000    | -0.0000    | -0.0000   | 0.0000    | 0.0000    | -0.2253       |
| $\Delta E$ | -0.0183023 | -0.0005482 | 0.0000559 | 0.0000266 | 0.0000078 | -14.7471259   |

Table S16: Errors in positions of orbital density maxima in bohr for the Be atom computed with TASKCC and the regularized potential with various values of  $a$ . The values obtained with the Coulomb potential of the point nucleus are shown in the last column.

| Energy | $a = 1.0$ | $a = 2.0$ | $a = 3.0$ | $a = 5.0$ | $a = 7.0$ | point nucleus |
|--------|-----------|-----------|-----------|-----------|-----------|---------------|
| 1s     | -0.002540 | -0.001765 | -0.000019 | 0.000000  | 0.000000  | 0.265586      |
| 2s     | 0.000682  | -0.000123 | -0.000012 | 0.000001  | 0.000001  | 2.108092      |



Table S17: Errors in orbital energies in  $E_h$  for the Ne atom computed with HF and the regularized potential with various values of  $a$ . The values obtained with the Coulomb potential of the point nucleus are shown in the last column. For comparison, the last row shows the errors in total energy  $\Delta E$  from the point nucleus value shown in the last column.

| Energy     | $a = 1.0$ | $a = 2.0$  | $a = 3.0$  | $a = 5.0$  | $a = 7.0$  | point nucleus |
|------------|-----------|------------|------------|------------|------------|---------------|
| 1s         | -0.1358   | -0.0087    | -0.0014    | -0.0001    | -0.0000    | -32.7724      |
| 2s         | 0.0002    | -0.0006    | -0.0001    | -0.0000    | -0.0000    | -1.9304       |
| 2p         | 0.0026    | 0.0002     | 0.0000     | 0.0000     | 0.0000     | -0.8504       |
| $\Delta E$ | 0.0523800 | -0.0004377 | -0.0001747 | -0.0000102 | -0.0000001 | -128.5470981  |

Table S18: Errors in positions of orbital density maxima in bohr for the Ne atom computed with HF and the regularized potential with various values of  $a$ . The values obtained with the Coulomb potential of the point nucleus are shown in the last column.

| Energy | $a = 1.0$ | $a = 2.0$ | $a = 3.0$ | $a = 5.0$ | $a = 7.0$ | point nucleus |
|--------|-----------|-----------|-----------|-----------|-----------|---------------|
| 1s     | -0.000052 | -0.000767 | -0.000009 | -0.000000 | -0.000000 | 0.102961      |
| 2s     | 0.001802  | -0.000016 | -0.000008 | -0.000001 | -0.000000 | 0.682866      |
| 2p     | 0.004276  | 0.000218  | 0.000034  | 0.000003  | 0.000001  | 0.634034      |

Table S19: Errors in orbital energies in  $E_h$  for the Ne atom computed with PW92 and the regularized potential with various values of  $a$ . The values obtained with the Coulomb potential of the point nucleus are shown in the last column. For comparison, the last row shows the errors in total energy  $\Delta E$  from the point nucleus value shown in the last column.

| Energy     | $a = 1.0$ | $a = 2.0$ | $a = 3.0$ | $a = 5.0$ | $a = 7.0$ | point nucleus |
|------------|-----------|-----------|-----------|-----------|-----------|---------------|
| 1s         | -0.1538   | -0.0089   | -0.0012   | -0.0001   | -0.0000   | -30.3058      |
| 2s         | -0.0016   | -0.0005   | -0.0001   | -0.0000   | -0.0000   | -1.3226       |
| 2p         | 0.0012    | 0.0001    | 0.0000    | 0.0000    | 0.0000    | -0.4978       |
| $\Delta E$ | 0.0619536 | 0.0024657 | 0.0006697 | 0.0001180 | 0.0000320 | -128.2299172  |

Table S20: Errors in positions of orbital density maxima in bohr for the Ne atom computed with PW92 and the regularized potential with various values of  $a$ . The values obtained with the Coulomb potential of the point nucleus are shown in the last column.

| Energy | $a = 1.0$ | $a = 2.0$ | $a = 3.0$ | $a = 5.0$ | $a = 7.0$ | point nucleus |
|--------|-----------|-----------|-----------|-----------|-----------|---------------|
| 1s     | -0.000147 | -0.000763 | -0.000009 | -0.000000 | 0.000000  | 0.103303      |
| 2s     | 0.001621  | -0.000022 | -0.000007 | -0.000001 | -0.000000 | 0.684641      |
| 2p     | 0.004359  | 0.000225  | 0.000035  | 0.000003  | 0.000001  | 0.619414      |

Table S21: Errors in orbital energies in  $E_h$  for the Ne atom computed with PBE and the regularized potential with various values of  $a$ . The values obtained with the Coulomb potential of the point nucleus are shown in the last column. For comparison, the last row shows the errors in total energy  $\Delta E$  from the point nucleus value shown in the last column.

| Energy     | $a = 1.0$ | $a = 2.0$ | $a = 3.0$ | $a = 5.0$ | $a = 7.0$ | point nucleus |
|------------|-----------|-----------|-----------|-----------|-----------|---------------|
| 1s         | -0.1494   | -0.0077   | -0.0007   | 0.0001    | 0.0000    | -30.4893      |
| 2s         | -0.0008   | -0.0004   | -0.0001   | -0.0000   | 0.0000    | -1.3332       |
| 2p         | 0.0011    | 0.0001    | 0.0000    | 0.0000    | -0.0000   | -0.4905       |
| $\Delta E$ | 0.0871932 | 0.0079460 | 0.0026781 | 0.0006372 | 0.0002368 | -128.8664277  |

Table S22: Errors in positions of orbital density maxima in bohr for the Ne atom computed with PBE and the regularized potential with various values of  $a$ . The values obtained with the Coulomb potential of the point nucleus are shown in the last column.

| Energy | $a = 1.0$ | $a = 2.0$ | $a = 3.0$ | $a = 5.0$ | $a = 7.0$ | point nucleus |
|--------|-----------|-----------|-----------|-----------|-----------|---------------|
| 1s     | -0.000025 | -0.000775 | -0.000008 | 0.000000  | 0.000000  | 0.102852      |
| 2s     | 0.001786  | 0.000001  | 0.000000  | 0.000001  | 0.000001  | 0.682308      |
| 2p     | 0.004281  | 0.000218  | 0.000033  | 0.000003  | 0.000000  | 0.622366      |

Table S23: Errors in orbital energies in  $E_h$  for the Ne atom computed with TASKCC and the regularized potential with various values of  $a$ . The values obtained with the Coulomb potential of the point nucleus are shown in the last column. For comparison, the last row shows the errors in total energy  $\Delta E$  from the point nucleus value shown in the last column.

| Energy     | $a = 1.0$ | $a = 2.0$ | $a = 3.0$ | $a = 5.0$ | $a = 7.0$ | point nucleus |
|------------|-----------|-----------|-----------|-----------|-----------|---------------|
| 1s         | -0.1474   | -0.0083   | -0.0011   | -0.0000   | -0.0000   | -30.7918      |
| 2s         | -0.0013   | -0.0005   | -0.0001   | -0.0000   | -0.0000   | -1.4406       |
| 2p         | 0.0013    | 0.0001    | 0.0000    | 0.0000    | 0.0000    | -0.5317       |
| $\Delta E$ | 0.0759949 | 0.0038248 | 0.0009306 | 0.0001417 | 0.0000352 | -128.9847733  |

Table S24: Errors in positions of orbital density maxima in bohr for the Ne atom computed with TASKCC and the regularized potential with various values of  $a$ . The values obtained with the Coulomb potential of the point nucleus are shown in the last column.

| Energy | $a = 1.0$ | $a = 2.0$ | $a = 3.0$ | $a = 5.0$ | $a = 7.0$ | point nucleus |
|--------|-----------|-----------|-----------|-----------|-----------|---------------|
| 1s     | -0.000008 | -0.000772 | -0.000009 | 0.000000  | 0.000000  | 0.102846      |
| 2s     | 0.001726  | -0.000009 | -0.000004 | -0.000000 | 0.000000  | 0.682910      |
| 2p     | 0.004459  | 0.000231  | 0.000035  | 0.000003  | 0.000001  | 0.627850      |

Table S25: Errors in orbital energies in  $E_h$  for the Mg atom computed with HF and the regularized potential with various values of  $a$ . The values obtained with the Coulomb potential of the point nucleus are shown in the last column. For comparison, the last row shows the errors in total energy  $\Delta E$  from the point nucleus value shown in the last column.

| Energy     | $a = 1.0$ | $a = 2.0$ | $a = 3.0$ | $a = 5.0$ | $a = 7.0$ | point nucleus |
|------------|-----------|-----------|-----------|-----------|-----------|---------------|
| 1s         | -0.1803   | -0.0115   | -0.0018   | -0.0001   | -0.0000   | -49.0317      |
| 2s         | 0.0067    | -0.0005   | -0.0001   | -0.0000   | -0.0000   | -3.7677       |
| 2p         | 0.0092    | 0.0006    | 0.0001    | 0.0000    | 0.0000    | -2.2822       |
| 3s         | 0.0004    | -0.0000   | -0.0000   | -0.0000   | -0.0000   | -0.2531       |
| $\Delta E$ | 0.1568757 | 0.0037706 | 0.0004204 | 0.0000414 | 0.0000103 | -199.6146364  |

Table S26: Errors in positions of orbital density maxima in bohr for the Mg atom computed with HF and the regularized potential with various values of  $a$ . The values obtained with the Coulomb potential of the point nucleus are shown in the last column.

| Energy | $a = 1.0$ | $a = 2.0$ | $a = 3.0$ | $a = 5.0$ | $a = 7.0$ | point nucleus |
|--------|-----------|-----------|-----------|-----------|-----------|---------------|
| 1s     | 0.000060  | -0.000645 | -0.000008 | -0.000000 | -0.000000 | 0.085455      |
| 2s     | 0.001786  | 0.000008  | -0.000003 | -0.000000 | -0.000000 | 0.546392      |
| 2p     | 0.003382  | 0.000174  | 0.000027  | 0.000002  | 0.000000  | 0.483857      |
| 3s     | 0.004245  | -0.000077 | -0.000029 | -0.000004 | -0.000001 | 2.585818      |

Table S27: Errors in orbital energies in  $E_h$  for the Mg atom computed with PW92 and the regularized potential with various values of  $a$ . The values obtained with the Coulomb potential of the point nucleus are shown in the last column. For comparison, the last row shows the errors in total energy  $\Delta E$  from the point nucleus value shown in the last column.

| Energy     | $a = 1.0$ | $a = 2.0$ | $a = 3.0$ | $a = 5.0$ | $a = 7.0$ | point nucleus |
|------------|-----------|-----------|-----------|-----------|-----------|---------------|
| 1s         | -0.2048   | -0.0119   | -0.0016   | -0.0001   | -0.0000   | -45.9730      |
| 2s         | 0.0038    | -0.0005   | -0.0001   | -0.0000   | -0.0000   | -2.9035       |
| 2p         | 0.0069    | 0.0005    | 0.0001    | 0.0000    | 0.0000    | -1.7187       |
| 3s         | 0.0002    | -0.0000   | -0.0000   | -0.0000   | -0.0000   | -0.1755       |
| $\Delta E$ | 0.1661910 | 0.0072293 | 0.0014451 | 0.0001984 | 0.0000498 | -199.1352883  |

Table S28: Errors in positions of orbital density maxima in bohr for the Mg atom computed with PW92 and the regularized potential with various values of  $a$ . The values obtained with the Coulomb potential of the point nucleus are shown in the last column.

| Energy | $a = 1.0$ | $a = 2.0$ | $a = 3.0$ | $a = 5.0$ | $a = 7.0$ | point nucleus |
|--------|-----------|-----------|-----------|-----------|-----------|---------------|
| 1s     | -0.000008 | -0.000643 | -0.000007 | -0.000000 | 0.000000  | 0.085699      |
| 2s     | 0.001663  | 0.000003  | -0.000003 | -0.000000 | 0.000000  | 0.549917      |
| 2p     | 0.003411  | 0.000177  | 0.000027  | 0.000002  | 0.000001  | 0.477654      |
| 3s     | 0.003501  | -0.000110 | -0.000030 | -0.000003 | 0.000000  | 2.518348      |

Table S29: Errors in orbital energies in  $E_h$  for the Mg atom computed with PBE and the regularized potential with various values of  $a$ . The values obtained with the Coulomb potential of the point nucleus are shown in the last column. For comparison, the last row shows the errors in total energy  $\Delta E$  from the point nucleus value shown in the last column.

| Energy     | $a = 1.0$ | $a = 2.0$ | $a = 3.0$ | $a = 5.0$ | $a = 7.0$ | point nucleus |
|------------|-----------|-----------|-----------|-----------|-----------|---------------|
| 1s         | -0.1988   | -0.0104   | -0.0010   | 0.0001    | 0.0001    | -46.2009      |
| 2s         | 0.0046    | -0.0004   | -0.0001   | 0.0000    | 0.0000    | -2.9235       |
| 2p         | 0.0065    | 0.0005    | 0.0001    | 0.0000    | 0.0000    | -1.7146       |
| 3s         | 0.0002    | -0.0000   | -0.0000   | 0.0000    | 0.0000    | -0.1727       |
| $\Delta E$ | 0.1985448 | 0.0141840 | 0.0039820 | 0.0008526 | 0.0003076 | -199.9551152  |

Table S30: Errors in positions of orbital density maxima in bohr for the Mg atom computed with PBE and the regularized potential with various values of  $a$ . The values obtained with the Coulomb potential of the point nucleus are shown in the last column.

| Energy | $a = 1.0$ | $a = 2.0$ | $a = 3.0$ | $a = 5.0$ | $a = 7.0$ | point nucleus |
|--------|-----------|-----------|-----------|-----------|-----------|---------------|
| 1s     | 0.000079  | -0.000651 | -0.000006 | 0.000000  | 0.000000  | 0.085382      |
| 2s     | 0.001767  | 0.000018  | 0.000002  | 0.000001  | 0.000000  | 0.548158      |
| 2p     | 0.003376  | 0.000174  | 0.000026  | 0.000002  | 0.000000  | 0.479202      |
| 3s     | 0.004042  | -0.000051 | -0.000012 | 0.000002  | 0.000001  | 2.559083      |

Table S31: Errors in orbital energies in  $E_h$  for the Mg atom computed with TASKCC and the regularized potential with various values of  $a$ . The values obtained with the Coulomb potential of the point nucleus are shown in the last column. For comparison, the last row shows the errors in total energy  $\Delta E$  from the point nucleus value shown in the last column.

| Energy     | $a = 1.0$ | $a = 2.0$ | $a = 3.0$ | $a = 5.0$ | $a = 7.0$ | point nucleus |
|------------|-----------|-----------|-----------|-----------|-----------|---------------|
| $1s$       | -0.1945   | -0.0112   | -0.0015   | -0.0001   | -0.0000   | -46.6129      |
| $2s$       | 0.0044    | -0.0005   | -0.0001   | -0.0000   | -0.0000   | -3.1041       |
| $2p$       | 0.0072    | 0.0005    | 0.0001    | 0.0000    | 0.0000    | -1.8254       |
| $3s$       | 0.0002    | -0.0000   | -0.0000   | -0.0000   | -0.0000   | -0.1849       |
| $\Delta E$ | 0.1857753 | 0.0090901 | 0.0017925 | 0.0002294 | 0.0000540 | -200.0383120  |

Table S32: Errors in positions of orbital density maxima in bohr for the Mg atom computed with TASKCC and the regularized potential with various values of  $a$ . The values obtained with the Coulomb potential of the point nucleus are shown in the last column.

| Energy | $a = 1.0$ | $a = 2.0$ | $a = 3.0$ | $a = 5.0$ | $a = 7.0$ | point nucleus |
|--------|-----------|-----------|-----------|-----------|-----------|---------------|
| $1s$   | 0.000085  | -0.000649 | -0.000007 | -0.000000 | 0.000000  | 0.085395      |
| $2s$   | 0.001738  | 0.000012  | -0.000001 | -0.000000 | 0.000000  | 0.548447      |
| $2p$   | 0.003458  | 0.000181  | 0.000028  | 0.000002  | 0.000000  | 0.480783      |
| $3s$   | 0.004261  | -0.000094 | -0.000027 | -0.000002 | 0.000000  | 2.713031      |

Table S33: Errors in orbital energies in  $E_h$  for the Ar atom computed with HF and the regularized potential with various values of  $a$ . The values obtained with the Coulomb potential of the point nucleus are shown in the last column. For comparison, the last row shows the errors in total energy  $\Delta E$  from the point nucleus value shown in the last column.

| Energy     | $a = 1.0$ | $a = 2.0$ | $a = 3.0$ | $a = 5.0$ | $a = 7.0$ | point nucleus |
|------------|-----------|-----------|-----------|-----------|-----------|---------------|
| 1s         | -0.3248   | -0.0214   | -0.0034   | -0.0003   | -0.0001   | -118.6104     |
| 2s         | 0.0490    | -0.0003   | -0.0002   | -0.0000   | -0.0000   | -12.3222      |
| 2p         | 0.0474    | 0.0027    | 0.0004    | 0.0000    | 0.0000    | -9.5715       |
| 3s         | 0.0044    | -0.0001   | -0.0000   | -0.0000   | -0.0000   | -1.2774       |
| 3p         | 0.0008    | 0.0001    | 0.0000    | 0.0000    | 0.0000    | -0.5910       |
| $\Delta E$ | 0.7641531 | 0.0315516 | 0.0045067 | 0.0003948 | 0.0000801 | -526.8175128  |

Table S34: Errors in positions of orbital density maxima in bohr for the Ar atom computed with HF and the regularized potential with various values of  $a$ . The values obtained with the Coulomb potential of the point nucleus are shown in the last column.

| Energy | $a = 1.0$ | $a = 2.0$ | $a = 3.0$ | $a = 5.0$ | $a = 7.0$ | point nucleus |
|--------|-----------|-----------|-----------|-----------|-----------|---------------|
| 1s     | 0.000161  | -0.000438 | -0.000005 | -0.000000 | -0.000000 | 0.056567      |
| 2s     | 0.001502  | 0.000028  | 0.000001  | -0.000000 | 0.000000  | 0.339084      |
| 2p     | 0.002093  | 0.000111  | 0.000018  | 0.000002  | 0.000000  | 0.282094      |
| 3s     | 0.003746  | 0.000045  | -0.000002 | 0.000000  | 0.000000  | 1.182481      |
| 3p     | 0.003496  | 0.000226  | 0.000038  | 0.000004  | 0.000001  | 1.299655      |

Table S35: Errors in orbital energies in  $E_h$  for the Ar atom computed with PW92 and the regularized potential with various values of  $a$ . The values obtained with the Coulomb potential of the point nucleus are shown in the last column. For comparison, the last row shows the errors in total energy  $\Delta E$  from the point nucleus value shown in the last column.

| Energy     | $a = 1.0$ | $a = 2.0$ | $a = 3.0$ | $a = 5.0$ | $a = 7.0$ | point nucleus |
|------------|-----------|-----------|-----------|-----------|-----------|---------------|
| 1s         | -0.3702   | -0.0226   | -0.0032   | -0.0002   | -0.0000   | -113.8001     |
| 2s         | 0.0410    | -0.0003   | -0.0002   | -0.0000   | -0.0000   | -10.7940      |
| 2p         | 0.0422    | 0.0024    | 0.0004    | 0.0000    | 0.0000    | -8.4433       |
| 3s         | 0.0032    | -0.0001   | -0.0000   | -0.0000   | -0.0000   | -0.8832       |
| 3p         | 0.0004    | 0.0001    | 0.0000    | 0.0000    | 0.0000    | -0.3822       |
| $\Delta E$ | 0.7709388 | 0.0366550 | 0.0060785 | 0.0006401 | 0.0001421 | -525.9397934  |

Table S36: Errors in positions of orbital density maxima in bohr for the Ar atom computed with PW92 and the regularized potential with various values of  $a$ . The values obtained with the Coulomb potential of the point nucleus are shown in the last column.

| Energy | $a = 1.0$ | $a = 2.0$ | $a = 3.0$ | $a = 5.0$ | $a = 7.0$ | point nucleus |
|--------|-----------|-----------|-----------|-----------|-----------|---------------|
| 1s     | 0.000130  | -0.000436 | -0.000005 | -0.000000 | 0.000000  | 0.056677      |
| 2s     | 0.001455  | 0.000026  | 0.000002  | 0.000000  | 0.000000  | 0.341584      |
| 2p     | 0.002100  | 0.000112  | 0.000018  | 0.000002  | 0.000000  | 0.281415      |
| 3s     | 0.003625  | 0.000030  | -0.000004 | -0.000001 | 0.000000  | 1.178438      |
| 3p     | 0.003447  | 0.000234  | 0.000039  | 0.000003  | 0.000001  | 1.288244      |

Table S37: Errors in orbital energies in  $E_h$  for the Ar atom computed with PBE and the regularized potential with various values of  $a$ . The values obtained with the Coulomb potential of the point nucleus are shown in the last column. For comparison, the last row shows the errors in total energy  $\Delta E$  from the point nucleus value shown in the last column.

| Energy     | $a = 1.0$ | $a = 2.0$ | $a = 3.0$ | $a = 5.0$ | $a = 7.0$ | point nucleus |
|------------|-----------|-----------|-----------|-----------|-----------|---------------|
| 1s         | -0.3587   | -0.0198   | -0.0021   | 0.0001    | 0.0001    | -114.1646     |
| 2s         | 0.0429    | -0.0001   | -0.0001   | 0.0000    | 0.0000    | -10.8310      |
| 2p         | 0.0417    | 0.0023    | 0.0004    | 0.0000    | 0.0000    | -8.4437       |
| 3s         | 0.0034    | -0.0001   | -0.0000   | -0.0000   | 0.0000    | -0.8842       |
| 3p         | 0.0003    | 0.0001    | 0.0000    | 0.0000    | 0.0000    | -0.3780       |
| $\Delta E$ | 0.8258155 | 0.0481923 | 0.0102538 | 0.0017119 | 0.0005641 | -527.3461288  |

Table S38: Errors in positions of orbital density maxima in bohr for the Ar atom computed with PBE and the regularized potential with various values of  $a$ . The values obtained with the Coulomb potential of the point nucleus are shown in the last column.

| Energy | $a = 1.0$ | $a = 2.0$ | $a = 3.0$ | $a = 5.0$ | $a = 7.0$ | point nucleus |
|--------|-----------|-----------|-----------|-----------|-----------|---------------|
| 1s     | 0.000169  | -0.000440 | -0.000005 | 0.000000  | 0.000000  | 0.056535      |
| 2s     | 0.001493  | 0.000032  | 0.000003  | 0.000001  | 0.000000  | 0.340626      |
| 2p     | 0.002093  | 0.000111  | 0.000017  | 0.000002  | 0.000000  | 0.281656      |
| 3s     | 0.003753  | 0.000051  | 0.000002  | 0.000000  | 0.000000  | 1.181186      |
| 3p     | 0.003433  | 0.000227  | 0.000037  | 0.000003  | 0.000000  | 1.292594      |

Table S39: Errors in orbital energies in  $E_h$  for the Ar atom computed with TASKCC and the regularized potential with various values of  $a$ . The values obtained with the Coulomb potential of the point nucleus are shown in the last column. For comparison, the last row shows the errors in total energy  $\Delta E$  from the point nucleus value shown in the last column.

| Energy     | $a = 1.0$ | $a = 2.0$ | $a = 3.0$ | $a = 5.0$ | $a = 7.0$ | point nucleus |
|------------|-----------|-----------|-----------|-----------|-----------|---------------|
| 1s         | -0.3474   | -0.0211   | -0.0029   | -0.0002   | -0.0000   | -114.7941     |
| 2s         | 0.0432    | -0.0002   | -0.0002   | -0.0000   | -0.0000   | -11.0871      |
| 2p         | 0.0429    | 0.0025    | 0.0004    | 0.0000    | 0.0000    | -8.6358       |
| 3s         | 0.0035    | -0.0001   | -0.0000   | -0.0000   | -0.0000   | -0.9492       |
| 3p         | 0.0004    | 0.0001    | 0.0000    | 0.0000    | 0.0000    | -0.4104       |
| $\Delta E$ | 0.8067793 | 0.0400977 | 0.0066984 | 0.0006937 | 0.0001493 | -527.3566109  |

Table S40: Errors in positions of orbital density maxima in bohr for the Ar atom computed with TASKCC and the regularized potential with various values of  $a$ . The values obtained with the Coulomb potential of the point nucleus are shown in the last column.

| Energy | $a = 1.0$ | $a = 2.0$ | $a = 3.0$ | $a = 5.0$ | $a = 7.0$ | point nucleus |
|--------|-----------|-----------|-----------|-----------|-----------|---------------|
| 1s     | 0.000167  | -0.000439 | -0.000005 | -0.000000 | 0.000000  | 0.056557      |
| 2s     | 0.001489  | 0.000030  | 0.000002  | 0.000000  | 0.000000  | 0.340711      |
| 2p     | 0.002103  | 0.000113  | 0.000018  | 0.000001  | 0.000000  | 0.281575      |
| 3s     | 0.003778  | 0.000053  | 0.000000  | 0.000000  | 0.000000  | 1.189354      |
| 3p     | 0.003506  | 0.000233  | 0.000038  | 0.000003  | 0.000001  | 1.300650      |

Table S41: Errors in orbital energies in  $E_h$  for the Ca atom computed with HF and the regularized potential with various values of  $a$ . The values obtained with the Coulomb potential of the point nucleus are shown in the last column. For comparison, the last row shows the errors in total energy  $\Delta E$  from the point nucleus value shown in the last column.

| Energy     | $a = 1.0$ | $a = 2.0$ | $a = 3.0$ | $a = 5.0$ | $a = 7.0$ | point nucleus |
|------------|-----------|-----------|-----------|-----------|-----------|---------------|
| $1s$       | -0.3752   | -0.0249   | -0.0040   | -0.0003   | -0.0001   | -149.3637     |
| $2s$       | 0.0727    | 0.0001    | -0.0002   | -0.0000   | -0.0000   | -16.8227      |
| $2p$       | 0.0681    | 0.0039    | 0.0006    | 0.0001    | 0.0000    | -13.6293      |
| $3s$       | 0.0084    | -0.0000   | -0.0000   | -0.0000   | -0.0000   | -2.2454       |
| $3p$       | 0.0023    | 0.0003    | 0.0001    | 0.0000    | 0.0000    | -1.3407       |
| $4s$       | 0.0004    | -0.0000   | -0.0000   | -0.0000   | -0.0000   | -0.1955       |
| $\Delta E$ | 1.0751494 | 0.0464898 | 0.0067317 | 0.0005870 | 0.0001178 | -676.7581859  |

Table S42: Errors in positions of orbital density maxima in bohr for the Ca atom computed with HF and the regularized potential with various values of  $a$ . The values obtained with the Coulomb potential of the point nucleus are shown in the last column.

| Energy | $a = 1.0$ | $a = 2.0$ | $a = 3.0$ | $a = 5.0$ | $a = 7.0$ | point nucleus |
|--------|-----------|-----------|-----------|-----------|-----------|---------------|
| $1s$   | 0.000168  | -0.000395 | -0.000005 | -0.000000 | -0.000000 | 0.050834      |
| $2s$   | 0.001406  | 0.000029  | 0.000002  | 0.000000  | 0.000000  | 0.300791      |
| $2p$   | 0.001856  | 0.000099  | 0.000016  | 0.000001  | 0.000000  | 0.247673      |
| $3s$   | 0.003418  | 0.000057  | 0.000001  | -0.000001 | -0.000000 | 0.996297      |
| $3p$   | 0.002991  | 0.000193  | 0.000032  | 0.000003  | 0.000001  | 1.052815      |
| $4s$   | 0.007769  | -0.000005 | -0.000027 | -0.000004 | -0.000001 | 3.475278      |

Table S43: Errors in orbital energies in  $E_h$  for the Ca atom computed with PW92 and the regularized potential with various values of  $a$ . The values obtained with the Coulomb potential of the point nucleus are shown in the last column. For comparison, the last row shows the errors in total energy  $\Delta E$  from the point nucleus value shown in the last column.

| Energy     | $a = 1.0$ | $a = 2.0$ | $a = 3.0$ | $a = 5.0$ | $a = 7.0$ | point nucleus |
|------------|-----------|-----------|-----------|-----------|-----------|---------------|
| $1s$       | -0.4281   | -0.0264   | -0.0038   | -0.0002   | -0.0000   | -143.9351     |
| $2s$       | 0.0626    | 0.0001    | -0.0002   | -0.0000   | -0.0000   | -15.0467      |
| $2p$       | 0.0617    | 0.0035    | 0.0006    | 0.0001    | 0.0000    | -12.2851      |
| $3s$       | 0.0065    | -0.0001   | -0.0000   | -0.0000   | -0.0000   | -1.7061       |
| $3p$       | 0.0016    | 0.0002    | 0.0000    | 0.0000    | 0.0000    | -1.0304       |
| $4s$       | 0.0002    | -0.0000   | -0.0000   | -0.0000   | -0.0000   | -0.1415       |
| $\Delta E$ | 1.0803757 | 0.0521100 | 0.0084837 | 0.0008620 | 0.0001874 | -675.7353039  |

Table S44: Errors in positions of orbital density maxima in bohr for the Ca atom computed with PW92 and the regularized potential with various values of  $a$ . The values obtained with the Coulomb potential of the point nucleus are shown in the last column.

| Energy | $a = 1.0$ | $a = 2.0$ | $a = 3.0$ | $a = 5.0$ | $a = 7.0$ | point nucleus |
|--------|-----------|-----------|-----------|-----------|-----------|---------------|
| 1s     | 0.000142  | -0.000394 | -0.000005 | -0.000000 | 0.000000  | 0.050924      |
| 2s     | 0.001367  | 0.000028  | 0.000002  | 0.000000  | 0.000000  | 0.302936      |
| 2p     | 0.001862  | 0.000100  | 0.000016  | 0.000001  | 0.000000  | 0.247380      |
| 3s     | 0.003356  | 0.000047  | -0.000000 | -0.000001 | -0.000000 | 0.998581      |
| 3p     | 0.002948  | 0.000196  | 0.000033  | 0.000003  | 0.000001  | 1.047653      |
| 4s     | 0.007202  | -0.000043 | -0.000031 | -0.000004 | -0.000001 | 3.340236      |

Table S45: Errors in orbital energies in  $E_h$  for the Ca atom computed with PBE and the regularized potential with various values of  $a$ . The values obtained with the Coulomb potential of the point nucleus are shown in the last column. For comparison, the last row shows the errors in total energy  $\Delta E$  from the point nucleus value shown in the last column.

| Energy     | $a = 1.0$ | $a = 2.0$ | $a = 3.0$ | $a = 5.0$ | $a = 7.0$ | point nucleus |
|------------|-----------|-----------|-----------|-----------|-----------|---------------|
| 1s         | -0.4147   | -0.0232   | -0.0025   | 0.0001    | 0.0001    | -144.3495     |
| 2s         | 0.0650    | 0.0004    | -0.0001   | 0.0000    | 0.0000    | -15.0918      |
| 2p         | 0.0611    | 0.0035    | 0.0006    | 0.0000    | 0.0000    | -12.2910      |
| 3s         | 0.0068    | -0.0000   | -0.0000   | -0.0000   | 0.0000    | -1.7157       |
| 3p         | 0.0015    | 0.0002    | 0.0000    | 0.0000    | 0.0000    | -1.0311       |
| 4s         | 0.0002    | 0.0000    | -0.0000   | -0.0000   | 0.0000    | -0.1379       |
| $\Delta E$ | 1.1431408 | 0.0652306 | 0.0132221 | 0.0020768 | 0.0006656 | -677.3488191  |

Table S46: Errors in positions of orbital density maxima in bohr for the Ca atom computed with PBE and the regularized potential with various values of  $a$ . The values obtained with the Coulomb potential of the point nucleus are shown in the last column.

| Energy | $a = 1.0$ | $a = 2.0$ | $a = 3.0$ | $a = 5.0$ | $a = 7.0$ | point nucleus |
|--------|-----------|-----------|-----------|-----------|-----------|---------------|
| 1s     | 0.000174  | -0.000397 | -0.000004 | 0.000000  | 0.000000  | 0.050808      |
| 2s     | 0.001397  | 0.000032  | 0.000004  | 0.000000  | 0.000000  | 0.302133      |
| 2p     | 0.001857  | 0.000099  | 0.000016  | 0.000001  | 0.000000  | 0.247512      |
| 3s     | 0.003440  | 0.000062  | 0.000005  | 0.000001  | 0.000000  | 0.999356      |
| 3p     | 0.002942  | 0.000192  | 0.000031  | 0.000002  | 0.000000  | 1.049867      |
| 4s     | 0.007684  | 0.000001  | -0.000018 | -0.000001 | 0.000000  | 3.413933      |



Table S47: Errors in orbital energies in  $E_h$  for the Ca atom computed with TASKCC and the regularized potential with various values of  $a$ . The values obtained with the Coulomb potential of the point nucleus are shown in the last column. For comparison, the last row shows the errors in total energy  $\Delta E$  from the point nucleus value shown in the last column.

| Energy     | $a = 1.0$ | $a = 2.0$ | $a = 3.0$ | $a = 5.0$ | $a = 7.0$ | point nucleus |
|------------|-----------|-----------|-----------|-----------|-----------|---------------|
| 1s         | -0.4009   | -0.0246   | -0.0034   | -0.0002   | -0.0000   | -145.0976     |
| 2s         | 0.0655    | 0.0002    | -0.0001   | -0.0000   | -0.0000   | -15.4188      |
| 2p         | 0.0626    | 0.0036    | 0.0006    | 0.0001    | 0.0000    | -12.5564      |
| 3s         | 0.0070    | -0.0000   | -0.0000   | -0.0000   | -0.0000   | -1.8348       |
| 3p         | 0.0016    | 0.0002    | 0.0000    | 0.0000    | 0.0000    | -1.1091       |
| 4s         | 0.0003    | 0.0000    | -0.0000   | -0.0000   | -0.0000   | -0.1454       |
| $\Delta E$ | 1.1216528 | 0.0561347 | 0.0092053 | 0.0009240 | 0.0001958 | -677.2532220  |

Table S48: Errors in positions of orbital density maxima in bohr for the Ca atom computed with TASKCC and the regularized potential with various values of  $a$ . The values obtained with the Coulomb potential of the point nucleus are shown in the last column.

| Energy | $a = 1.0$ | $a = 2.0$ | $a = 3.0$ | $a = 5.0$ | $a = 7.0$ | point nucleus |
|--------|-----------|-----------|-----------|-----------|-----------|---------------|
| 1s     | 0.000171  | -0.000396 | -0.000004 | -0.000000 | 0.000000  | 0.050830      |
| 2s     | 0.001395  | 0.000031  | 0.000003  | 0.000000  | 0.000000  | 0.302211      |
| 2p     | 0.001862  | 0.000101  | 0.000016  | 0.000001  | 0.000000  | 0.247389      |
| 3s     | 0.003451  | 0.000062  | 0.000003  | 0.000000  | 0.000000  | 1.003105      |
| 3p     | 0.002987  | 0.000197  | 0.000033  | 0.000003  | 0.000001  | 1.053457      |
| 4s     | 0.009015  | -0.000049 | -0.000038 | -0.000005 | -0.000001 | 3.669521      |

Table S49: Errors in orbital energies in  $E_h$  for the Zn atom computed with HF and the regularized potential with various values of  $a$ . The values obtained with the Coulomb potential of the point nucleus are shown in the last column. For comparison, the last row shows the errors in total energy  $\Delta E$  from the point nucleus value shown in the last column.

| Energy     | $a = 1.0$ | $a = 2.0$ | $a = 3.0$ | $a = 5.0$ | $a = 7.0$ | point nucleus |
|------------|-----------|-----------|-----------|-----------|-----------|---------------|
| 1s         | -0.5958   | -0.0409   | -0.0066   | -0.0005   | -0.0001   | -353.3045     |
| 2s         | 0.3070    | 0.0065    | 0.0004    | -0.0000   | -0.0000   | -44.3617      |
| 2p         | 0.2712    | 0.0155    | 0.0025    | 0.0002    | 0.0000    | -38.9248      |
| 3s         | 0.0590    | 0.0016    | 0.0001    | 0.0000    | 0.0000    | -5.6378       |
| 3p         | 0.0319    | 0.0023    | 0.0004    | 0.0000    | 0.0000    | -3.8394       |
| 3d         | -0.0107   | -0.0005   | -0.0001   | -0.0000   | -0.0000   | -0.7825       |
| 4s         | 0.0023    | 0.0001    | 0.0000    | 0.0000    | 0.0000    | -0.2925       |
| $\Delta E$ | 3.2644482 | 0.1556870 | 0.0231720 | 0.0020104 | 0.0003960 | -1777.8481162 |

Table S50: Errors in positions of orbital density maxima in bohr for the Zn atom computed with HF and the regularized potential with various values of  $a$ . The values obtained with the Coulomb potential of the point nucleus are shown in the last column.

| Energy | $a = 1.0$ | $a = 2.0$ | $a = 3.0$ | $a = 5.0$ | $a = 7.0$ | point nucleus |
|--------|-----------|-----------|-----------|-----------|-----------|---------------|
| 1s     | 0.000161  | -0.000266 | -0.000003 | -0.000000 | -0.000000 | 0.033722      |
| 2s     | 0.001056  | 0.000028  | 0.000002  | 0.000000  | 0.000000  | 0.191985      |
| 2p     | 0.001191  | 0.000066  | 0.000010  | 0.000001  | 0.000000  | 0.153583      |
| 3s     | 0.003081  | 0.000086  | 0.000008  | 0.000000  | 0.000000  | 0.596687      |
| 3p     | 0.002474  | 0.000161  | 0.000027  | 0.000003  | 0.000000  | 0.598608      |
| 3d     | -0.001338 | -0.000078 | -0.000012 | -0.000001 | -0.000000 | 0.573959      |
| 4s     | 0.016189  | 0.000505  | 0.000052  | 0.000002  | 0.000000  | 2.267465      |

Table S51: Errors in orbital energies in  $E_h$  for the Zn atom computed with PW92 and the regularized potential with various values of  $a$ . The values obtained with the Coulomb potential of the point nucleus are shown in the last column. For comparison, the last row shows the errors in total energy  $\Delta E$  from the point nucleus value shown in the last column.

| Energy     | $a = 1.0$ | $a = 2.0$ | $a = 3.0$ | $a = 5.0$ | $a = 7.0$ | point nucleus |
|------------|-----------|-----------|-----------|-----------|-----------|---------------|
| 1s         | -0.6860   | -0.0440   | -0.0064   | -0.0004   | -0.0001   | -344.9698     |
| 2s         | 0.2881    | 0.0063    | 0.0005    | 0.0000    | -0.0000   | -41.5313      |
| 2p         | 0.2619    | 0.0150    | 0.0024    | 0.0002    | 0.0000    | -36.6487      |
| 3s         | 0.0545    | 0.0015    | 0.0001    | 0.0000    | 0.0000    | -4.5729       |
| 3p         | 0.0305    | 0.0022    | 0.0004    | 0.0000    | 0.0000    | -3.0222       |
| 3d         | -0.0074   | -0.0003   | -0.0000   | -0.0000   | -0.0000   | -0.3988       |
| 4s         | 0.0022    | 0.0001    | 0.0000    | 0.0000    | 0.0000    | -0.2227       |
| $\Delta E$ | 3.2655204 | 0.1640487 | 0.0258466 | 0.0024352 | 0.0005039 | -1776.5614778 |

Table S52: Errors in positions of orbital density maxima in bohr for the Zn atom computed with PW92 and the regularized potential with various values of  $a$ . The values obtained with the Coulomb potential of the point nucleus are shown in the last column.

| Energy | $a = 1.0$ | $a = 2.0$ | $a = 3.0$ | $a = 5.0$ | $a = 7.0$ | point nucleus |
|--------|-----------|-----------|-----------|-----------|-----------|---------------|
| 1s     | 0.000150  | -0.000266 | -0.000003 | -0.000000 | 0.000000  | 0.033761      |
| 2s     | 0.001037  | 0.000027  | 0.000003  | 0.000000  | 0.000000  | 0.192868      |
| 2p     | 0.001188  | 0.000066  | 0.000010  | 0.000001  | 0.000000  | 0.153474      |
| 3s     | 0.003085  | 0.000083  | 0.000008  | 0.000000  | 0.000000  | 0.597388      |
| 3p     | 0.002480  | 0.000165  | 0.000027  | 0.000003  | 0.000001  | 0.595704      |
| 3d     | -0.001335 | -0.000080 | -0.000012 | -0.000001 | -0.000000 | 0.562133      |
| 4s     | 0.014769  | 0.000463  | 0.000050  | 0.000003  | 0.000001  | 2.115892      |

Table S53: Errors in orbital energies in  $E_h$  for the Zn atom computed with PBE and the regularized potential with various values of  $a$ . The values obtained with the Coulomb potential of the point nucleus are shown in the last column. For comparison, the last row shows the errors in total energy  $\Delta E$  from the point nucleus value shown in the last column.

| Energy     | $a = 1.0$ | $a = 2.0$ | $a = 3.0$ | $a = 5.0$ | $a = 7.0$ | point nucleus |
|------------|-----------|-----------|-----------|-----------|-----------|---------------|
| 1s         | -0.6625   | -0.0385   | -0.0043   | 0.0001    | 0.0002    | -345.6328     |
| 2s         | 0.2928    | 0.0070    | 0.0007    | 0.0001    | 0.0000    | -41.6065      |
| 2p         | 0.2613    | 0.0149    | 0.0024    | 0.0002    | 0.0000    | -36.6697      |
| 3s         | 0.0554    | 0.0016    | 0.0002    | 0.0000    | 0.0000    | -4.5946       |
| 3p         | 0.0304    | 0.0022    | 0.0004    | 0.0000    | 0.0000    | -3.0271       |
| 3d         | -0.0074   | -0.0003   | -0.0000   | -0.0000   | -0.0000   | -0.3883       |
| 4s         | 0.0022    | 0.0001    | 0.0000    | 0.0000    | 0.0000    | -0.2141       |
| $\Delta E$ | 3.3690056 | 0.1851807 | 0.0334234 | 0.0043699 | 0.0012647 | -1779.1827967 |

Table S54: Errors in positions of orbital density maxima in bohr for the Zn atom computed with PBE and the regularized potential with various values of  $a$ . The values obtained with the Coulomb potential of the point nucleus are shown in the last column.

| Energy | $a = 1.0$ | $a = 2.0$ | $a = 3.0$ | $a = 5.0$ | $a = 7.0$ | point nucleus |
|--------|-----------|-----------|-----------|-----------|-----------|---------------|
| 1s     | 0.000164  | -0.000267 | -0.000003 | 0.000000  | 0.000000  | 0.033710      |
| 2s     | 0.001051  | 0.000029  | 0.000003  | 0.000000  | 0.000000  | 0.192522      |
| 2p     | 0.001188  | 0.000066  | 0.000010  | 0.000001  | 0.000000  | 0.153485      |
| 3s     | 0.003111  | 0.000089  | 0.000009  | 0.000001  | 0.000000  | 0.596809      |
| 3p     | 0.002473  | 0.000164  | 0.000027  | 0.000003  | 0.000000  | 0.595945      |
| 3d     | -0.001295 | -0.000078 | -0.000012 | -0.000001 | -0.000000 | 0.564979      |
| 4s     | 0.015642  | 0.000517  | 0.000061  | 0.000005  | 0.000001  | 2.131212      |

Table S55: Errors in orbital energies in  $E_h$  for the Zn atom computed with TASKCC and the regularized potential with various values of  $a$ . The values obtained with the Coulomb potential of the point nucleus are shown in the last column. For comparison, the last row shows the errors in total energy  $\Delta E$  from the point nucleus value shown in the last column.

| Energy     | $a = 1.0$ | $a = 2.0$ | $a = 3.0$ | $a = 5.0$ | $a = 7.0$ | point nucleus |
|------------|-----------|-----------|-----------|-----------|-----------|---------------|
| 1s         | -0.6377   | -0.0407   | -0.0057   | -0.0003   | -0.0000   | -346.6925     |
| 2s         | 0.2933    | 0.0067    | 0.0005    | 0.0000    | 0.0000    | -42.0686      |
| 2p         | 0.2627    | 0.0152    | 0.0024    | 0.0002    | 0.0000    | -37.0495      |
| 3s         | 0.0555    | 0.0016    | 0.0002    | 0.0000    | 0.0000    | -4.7832       |
| 3p         | 0.0302    | 0.0022    | 0.0004    | 0.0000    | 0.0000    | -3.1623       |
| 3d         | -0.0083   | -0.0004   | -0.0001   | -0.0000   | -0.0000   | -0.4067       |
| 4s         | 0.0028    | 0.0001    | 0.0000    | 0.0000    | 0.0000    | -0.2374       |
| $\Delta E$ | 3.3280591 | 0.1705826 | 0.0270148 | 0.0025340 | 0.0005172 | -1778.7847235 |

Table S56: Errors in positions of orbital density maxima in bohr for the Zn atom computed with TASKCC and the regularized potential with various values of  $a$ . The values obtained with the Coulomb potential of the point nucleus are shown in the last column.

| Energy | $a = 1.0$ | $a = 2.0$ | $a = 3.0$ | $a = 5.0$ | $a = 7.0$ | point nucleus |
|--------|-----------|-----------|-----------|-----------|-----------|---------------|
| 1s     | 0.000162  | -0.000267 | -0.000003 | -0.000000 | 0.000000  | 0.033723      |
| 2s     | 0.001052  | 0.000029  | 0.000003  | 0.000000  | 0.000000  | 0.192629      |
| 2p     | 0.001189  | 0.000067  | 0.000011  | 0.000001  | 0.000000  | 0.153492      |
| 3s     | 0.003118  | 0.000087  | 0.000008  | 0.000000  | 0.000000  | 0.598052      |
| 3p     | 0.002476  | 0.000165  | 0.000027  | 0.000003  | 0.000001  | 0.597291      |
| 3d     | -0.001267 | -0.000077 | -0.000012 | -0.000001 | -0.000000 | 0.567963      |
| 4s     | 0.018627  | 0.000625  | 0.000072  | 0.000005  | 0.000001  | 2.157472      |

Table S57: Errors in orbital energies in  $E_h$  for the Kr atom computed with HF and the regularized potential with various values of  $a$ . The values obtained with the Coulomb potential of the point nucleus are shown in the last column. For comparison, the last row shows the errors in total energy  $\Delta E$  from the point nucleus value shown in the last column.

| Energy     | $a = 1.0$ | $a = 2.0$ | $a = 3.0$ | $a = 5.0$ | $a = 7.0$ | point nucleus |
|------------|-----------|-----------|-----------|-----------|-----------|---------------|
| 1s         | -0.7542   | -0.0523   | -0.0084   | -0.0007   | -0.0001   | -520.1655     |
| 2s         | 0.4881    | 0.0111    | 0.0007    | -0.0000   | -0.0000   | -69.9031      |
| 2p         | 0.4215    | 0.0243    | 0.0039    | 0.0004    | 0.0001    | -63.0098      |
| 3s         | 0.0923    | 0.0022    | 0.0001    | -0.0000   | -0.0000   | -10.8495      |
| 3p         | 0.0448    | 0.0033    | 0.0006    | 0.0001    | 0.0000    | -8.3315       |
| 3d         | -0.0313   | -0.0018   | -0.0003   | -0.0000   | -0.0000   | -3.8252       |
| 4s         | 0.0075    | 0.0001    | -0.0000   | -0.0000   | -0.0000   | -1.1529       |
| 4p         | 0.0005    | 0.0001    | 0.0000    | 0.0000    | 0.0000    | -0.5242       |
| $\Delta E$ | 5.2478688 | 0.2572838 | 0.0385769 | 0.0033455 | 0.0006563 | -2752.0549773 |

Table S58: Errors in positions of orbital density maxima in bohr for the Kr atom computed with HF and the regularized potential with various values of  $a$ . The values obtained with the Coulomb potential of the point nucleus are shown in the last column.

| Energy | $a = 1.0$ | $a = 2.0$ | $a = 3.0$ | $a = 5.0$ | $a = 7.0$ | point nucleus |
|--------|-----------|-----------|-----------|-----------|-----------|---------------|
| $1s$   | 0.000149  | -0.000223 | -0.000003 | -0.000000 | 0.000000  | 0.028053      |
| $2s$   | 0.000912  | 0.000025  | 0.000002  | 0.000000  | 0.000000  | 0.157808      |
| $2p$   | 0.000980  | 0.000055  | 0.000009  | 0.000001  | 0.000000  | 0.125184      |
| $3s$   | 0.002485  | 0.000072  | 0.000007  | 0.000000  | 0.000000  | 0.475424      |
| $3p$   | 0.001813  | 0.000122  | 0.000020  | 0.000002  | 0.000000  | 0.467508      |
| $3d$   | -0.000627 | -0.000040 | -0.000006 | -0.000000 | -0.000000 | 0.413214      |
| $4s$   | 0.006377  | 0.000164  | 0.000012  | 0.000000  | 0.000000  | 1.376905      |
| $4p$   | 0.004037  | 0.000304  | 0.000052  | 0.000005  | 0.000001  | 1.565641      |

Table S59: Errors in orbital energies in  $E_h$  for the Kr atom computed with PW92 and the regularized potential with various values of  $a$ . The values obtained with the Coulomb potential of the point nucleus are shown in the last column. For comparison, the last row shows the errors in total energy  $\Delta E$  from the point nucleus value shown in the last column.

| Energy     | $a = 1.0$ | $a = 2.0$ | $a = 3.0$ | $a = 5.0$ | $a = 7.0$ | point nucleus |
|------------|-----------|-----------|-----------|-----------|-----------|---------------|
| $1s$       | -0.8679   | -0.0564   | -0.0082   | -0.0006   | -0.0001   | -509.9831     |
| $2s$       | 0.4627    | 0.0108    | 0.0008    | 0.0000    | -0.0000   | -66.2859      |
| $2p$       | 0.4095    | 0.0235    | 0.0038    | 0.0003    | 0.0001    | -60.0173      |
| $3s$       | 0.0835    | 0.0019    | 0.0001    | -0.0000   | -0.0000   | -9.3150       |
| $3p$       | 0.0403    | 0.0030    | 0.0005    | 0.0000    | 0.0000    | -7.0865       |
| $3d$       | -0.0289   | -0.0017   | -0.0003   | -0.0000   | -0.0000   | -3.0739       |
| $4s$       | 0.0065    | 0.0000    | -0.0000   | -0.0000   | -0.0000   | -0.8205       |
| $4p$       | 0.0002    | 0.0001    | 0.0000    | 0.0000    | 0.0000    | -0.3463       |
| $\Delta E$ | 5.2403164 | 0.2670035 | 0.0417684 | 0.0038580 | 0.0007869 | -2750.1333061 |

Table S60: Errors in positions of orbital density maxima in bohr for the Kr atom computed with PW92 and the regularized potential with various values of  $a$ . The values obtained with the Coulomb potential of the point nucleus are shown in the last column.

| Energy | $a = 1.0$ | $a = 2.0$ | $a = 3.0$ | $a = 5.0$ | $a = 7.0$ | point nucleus |
|--------|-----------|-----------|-----------|-----------|-----------|---------------|
| $1s$   | 0.000141  | -0.000222 | -0.000003 | -0.000000 | 0.000000  | 0.028081      |
| $2s$   | 0.000898  | 0.000025  | 0.000002  | 0.000000  | 0.000000  | 0.158392      |
| $2p$   | 0.000977  | 0.000055  | 0.000009  | 0.000001  | 0.000000  | 0.125108      |
| $3s$   | 0.002518  | 0.000072  | 0.000007  | 0.000000  | 0.000000  | 0.477492      |
| $3p$   | 0.001835  | 0.000125  | 0.000021  | 0.000002  | 0.000000  | 0.467632      |
| $3d$   | -0.000627 | -0.000041 | -0.000007 | -0.000001 | -0.000000 | 0.409450      |
| $4s$   | 0.006505  | 0.000153  | 0.000011  | 0.000000  | 0.000000  | 1.359649      |
| $4p$   | 0.003924  | 0.000318  | 0.000055  | 0.000006  | 0.000001  | 1.553438      |

Table S61: Errors in orbital energies in  $E_h$  for the Kr atom computed with PBE and the regularized potential with various values of  $a$ . The values obtained with the Coulomb potential of the point nucleus are shown in the last column. For comparison, the last row shows the errors in total energy  $\Delta E$  from the point nucleus value shown in the last column.

| Energy     | $a = 1.0$ | $a = 2.0$ | $a = 3.0$ | $a = 5.0$ | $a = 7.0$ | point nucleus |
|------------|-----------|-----------|-----------|-----------|-----------|---------------|
| 1s         | -0.8382   | -0.0496   | -0.0057   | 0.0001    | 0.0002    | -510.7930     |
| 2s         | 0.4689    | 0.0116    | 0.0011    | 0.0001    | 0.0000    | -66.3746      |
| 2p         | 0.4090    | 0.0235    | 0.0038    | 0.0003    | 0.0001    | -60.0432      |
| 3s         | 0.0849    | 0.0021    | 0.0002    | 0.0000    | 0.0000    | -9.3468       |
| 3p         | 0.0404    | 0.0030    | 0.0005    | 0.0000    | 0.0000    | -7.0965       |
| 3d         | -0.0290   | -0.0017   | -0.0003   | -0.0000   | -0.0000   | -3.0630       |
| 4s         | 0.0065    | 0.0000    | -0.0000   | -0.0000   | -0.0000   | -0.8147       |
| 4p         | 0.0001    | 0.0000    | 0.0000    | 0.0000    | 0.0000    | -0.3411       |
| $\Delta E$ | 5.3681294 | 0.2929986 | 0.0510716 | 0.0062308 | 0.0017197 | -2753.4161089 |

Table S62: Errors in positions of orbital density maxima in bohr for the Kr atom computed with PBE and the regularized potential with various values of  $a$ . The values obtained with the Coulomb potential of the point nucleus are shown in the last column.

| Energy | $a = 1.0$ | $a = 2.0$ | $a = 3.0$ | $a = 5.0$ | $a = 7.0$ | point nucleus |
|--------|-----------|-----------|-----------|-----------|-----------|---------------|
| 1s     | 0.000151  | -0.000223 | -0.000002 | 0.000000  | 0.000000  | 0.028045      |
| 2s     | 0.000908  | 0.000026  | 0.000003  | 0.000000  | 0.000000  | 0.158157      |
| 2p     | 0.000977  | 0.000055  | 0.000009  | 0.000001  | 0.000000  | 0.125104      |
| 3s     | 0.002532  | 0.000075  | 0.000008  | 0.000001  | 0.000000  | 0.476901      |
| 3p     | 0.001829  | 0.000125  | 0.000021  | 0.000002  | 0.000000  | 0.467532      |
| 3d     | -0.000618 | -0.000040 | -0.000006 | -0.000001 | -0.000000 | 0.410773      |
| 4s     | 0.006655  | 0.000170  | 0.000015  | 0.000001  | 0.000000  | 1.366808      |
| 4p     | 0.003986  | 0.000315  | 0.000054  | 0.000005  | 0.000001  | 1.560857      |

Table S63: Errors in orbital energies in  $E_h$  for the Kr atom computed with TASKCC and the regularized potential with various values of  $a$ . The values obtained with the Coulomb potential of the point nucleus are shown in the last column. For comparison, the last row shows the errors in total energy  $\Delta E$  from the point nucleus value shown in the last column.

| Energy     | $a = 1.0$ | $a = 2.0$ | $a = 3.0$ | $a = 5.0$ | $a = 7.0$ | point nucleus |
|------------|-----------|-----------|-----------|-----------|-----------|---------------|
| 1s         | -0.8068   | -0.0522   | -0.0074   | -0.0005   | -0.0001   | -512.1085     |
| 2s         | 0.4693    | 0.0113    | 0.0009    | 0.0000    | 0.0000    | -67.0180      |
| 2p         | 0.4100    | 0.0238    | 0.0038    | 0.0003    | 0.0001    | -60.5880      |
| 3s         | 0.0860    | 0.0021    | 0.0001    | 0.0000    | -0.0000   | -9.6297       |
| 3p         | 0.0408    | 0.0031    | 0.0005    | 0.0000    | 0.0000    | -7.3197       |
| 3d         | -0.0299   | -0.0017   | -0.0003   | -0.0000   | -0.0000   | -3.1594       |
| 4s         | 0.0069    | 0.0000    | -0.0000   | -0.0000   | -0.0000   | -0.8760       |
| 4p         | 0.0001    | 0.0001    | 0.0000    | 0.0000    | 0.0000    | -0.3711       |
| $\Delta E$ | 5.3182805 | 0.2753149 | 0.0432544 | 0.0039834 | 0.0008039 | -2753.0465769 |

Table S64: Errors in positions of orbital density maxima in bohr for the Kr atom computed with TASKCC and the regularized potential with various values of  $a$ . The values obtained with the Coulomb potential of the point nucleus are shown in the last column.

| Energy | $a = 1.0$ | $a = 2.0$ | $a = 3.0$ | $a = 5.0$ | $a = 7.0$ | point nucleus |
|--------|-----------|-----------|-----------|-----------|-----------|---------------|
| $1s$   | 0.000149  | -0.000223 | -0.000003 | 0.000000  | 0.000000  | 0.028055      |
| $2s$   | 0.000909  | 0.000026  | 0.000003  | 0.000000  | 0.000000  | 0.158252      |
| $2p$   | 0.000977  | 0.000055  | 0.000009  | 0.000001  | 0.000000  | 0.125131      |
| $3s$   | 0.002528  | 0.000074  | 0.000007  | 0.000000  | 0.000000  | 0.477387      |
| $3p$   | 0.001820  | 0.000125  | 0.000021  | 0.000002  | 0.000000  | 0.467845      |
| $3d$   | -0.000611 | -0.000040 | -0.000006 | -0.000001 | -0.000000 | 0.411521      |
| $4s$   | 0.006835  | 0.000184  | 0.000016  | 0.000001  | 0.000000  | 1.376068      |
| $4p$   | 0.004248  | 0.000330  | 0.000057  | 0.000006  | 0.000001  | 1.562354      |

Table S65: Errors in orbital energies in  $E_h$  for the Sr atom computed with HF and the regularized potential with various values of  $a$ . The values obtained with the Coulomb potential of the point nucleus are shown in the last column. For comparison, the last row shows the errors in total energy  $\Delta E$  from the point nucleus value shown in the last column.

| Energy     | $a = 1.0$ | $a = 2.0$ | $a = 3.0$ | $a = 5.0$ | $a = 7.0$ | point nucleus |
|------------|-----------|-----------|-----------|-----------|-----------|---------------|
| 1s         | -0.8079   | -0.0561   | -0.0090   | -0.0008   | -0.0001   | -583.6879     |
| 2s         | 0.5597    | 0.0131    | 0.0009    | -0.0000   | -0.0000   | -80.3908      |
| 2p         | 0.4806    | 0.0278    | 0.0045    | 0.0004    | 0.0001    | -72.9960      |
| 3s         | 0.1081    | 0.0026    | 0.0002    | -0.0000   | -0.0000   | -13.4750      |
| 3p         | 0.0517    | 0.0039    | 0.0007    | 0.0001    | 0.0000    | -10.7000      |
| 3d         | -0.0380   | -0.0022   | -0.0003   | -0.0000   | -0.0000   | -5.6944       |
| 4s         | 0.0108    | 0.0002    | -0.0000   | -0.0000   | -0.0000   | -1.8968       |
| 4p         | 0.0010    | 0.0002    | 0.0000    | 0.0000    | 0.0000    | -1.0982       |
| 5s         | 0.0006    | 0.0000    | -0.0000   | -0.0000   | -0.0000   | -0.1785       |
| $\Delta E$ | 6.0345652 | 0.2979414 | 0.0447537 | 0.0038809 | 0.0007606 | -3131.5456864 |

Table S66: Errors in positions of orbital density maxima in bohr for the Sr atom computed with HF and the regularized potential with various values of  $a$ . The values obtained with the Coulomb potential of the point nucleus are shown in the last column.

| Energy | $a = 1.0$ | $a = 2.0$ | $a = 3.0$ | $a = 5.0$ | $a = 7.0$ | point nucleus |
|--------|-----------|-----------|-----------|-----------|-----------|---------------|
| 1s     | 0.000144  | -0.000211 | -0.000002 | -0.000000 | 0.000000  | 0.026565      |
| 2s     | 0.000872  | 0.000025  | 0.000002  | 0.000000  | 0.000000  | 0.148959      |
| 2p     | 0.000924  | 0.000052  | 0.000008  | 0.000001  | 0.000000  | 0.117913      |
| 3s     | 0.002328  | 0.000069  | 0.000007  | 0.000000  | 0.000000  | 0.444452      |
| 3p     | 0.001659  | 0.000113  | 0.000019  | 0.000002  | 0.000000  | 0.434878      |
| 3d     | -0.000506 | -0.000034 | -0.000005 | -0.000001 | -0.000000 | 0.378131      |
| 4s     | 0.005368  | 0.000143  | 0.000012  | 0.000000  | 0.000000  | 1.217484      |
| 4p     | 0.003311  | 0.000249  | 0.000042  | 0.000004  | 0.000000  | 1.337044      |
| 5s     | 0.012959  | 0.000174  | -0.000010 | -0.000004 | -0.000001 | 3.862631      |

Table S67: Errors in orbital energies in  $E_h$  for the Sr atom computed with PW92 and the regularized potential with various values of  $a$ . The values obtained with the Coulomb potential of the point nucleus are shown in the last column. For comparison, the last row shows the errors in total energy  $\Delta E$  from the point nucleus value shown in the last column.

| Energy     | $a = 1.0$ | $a = 2.0$ | $a = 3.0$ | $a = 5.0$ | $a = 7.0$ | point nucleus |
|------------|-----------|-----------|-----------|-----------|-----------|---------------|
| 1s         | -0.9295   | -0.0606   | -0.0088   | -0.0006   | -0.0001   | -572.8702     |
| 2s         | 0.5320    | 0.0127    | 0.0010    | 0.0000    | -0.0000   | -76.4916      |
| 2p         | 0.4677    | 0.0270    | 0.0044    | 0.0004    | 0.0001    | -69.7458      |
| 3s         | 0.0978    | 0.0023    | 0.0002    | -0.0000   | -0.0000   | -11.7713      |
| 3p         | 0.0463    | 0.0036    | 0.0006    | 0.0001    | 0.0000    | -9.3016       |
| 3d         | -0.0359   | -0.0020   | -0.0003   | -0.0000   | -0.0000   | -4.8132       |
| 4s         | 0.0094    | 0.0001    | -0.0000   | -0.0000   | -0.0000   | -1.4551       |
| 4p         | 0.0005    | 0.0002    | 0.0000    | 0.0000    | 0.0000    | -0.8443       |
| 5s         | 0.0004    | 0.0000    | -0.0000   | -0.0000   | -0.0000   | -0.1319       |
| $\Delta E$ | 6.0243861 | 0.3081219 | 0.0481193 | 0.0044229 | 0.0008988 | -3129.4380223 |



Table S68: Errors in positions of orbital density maxima in bohr for the Sr atom computed with PW92 and the regularized potential with various values of  $a$ . The values obtained with the Coulomb potential of the point nucleus are shown in the last column.

| Energy | $a = 1.0$ | $a = 2.0$ | $a = 3.0$ | $a = 5.0$ | $a = 7.0$ | point nucleus |
|--------|-----------|-----------|-----------|-----------|-----------|---------------|
| 1s     | 0.000137  | -0.000211 | -0.000002 | -0.000000 | 0.000000  | 0.026589      |
| 2s     | 0.000859  | 0.000024  | 0.000002  | 0.000000  | 0.000000  | 0.149479      |
| 2p     | 0.000922  | 0.000052  | 0.000008  | 0.000001  | 0.000000  | 0.117848      |
| 3s     | 0.002359  | 0.000068  | 0.000007  | 0.000000  | 0.000000  | 0.446670      |
| 3p     | 0.001678  | 0.000115  | 0.000019  | 0.000002  | 0.000000  | 0.435391      |
| 3d     | -0.000505 | -0.000034 | -0.000005 | -0.000001 | -0.000000 | 0.375268      |
| 4s     | 0.005517  | 0.000136  | 0.000010  | 0.000000  | 0.000000  | 1.211884      |
| 4p     | 0.003240  | 0.000257  | 0.000044  | 0.000004  | 0.000001  | 1.331663      |
| 5s     | 0.012516  | 0.000133  | -0.000015 | -0.000004 | -0.000001 | 3.678856      |

Table S69: Errors in orbital energies in  $E_h$  for the Sr atom computed with PBE and the regularized potential with various values of  $a$ . The values obtained with the Coulomb potential of the point nucleus are shown in the last column. For comparison, the last row shows the errors in total energy  $\Delta E$  from the point nucleus value shown in the last column.

| Energy     | $a = 1.0$ | $a = 2.0$ | $a = 3.0$ | $a = 5.0$ | $a = 7.0$ | point nucleus |
|------------|-----------|-----------|-----------|-----------|-----------|---------------|
| 1s         | -0.8978   | -0.0533   | -0.0061   | 0.0001    | 0.0002    | -573.7319     |
| 2s         | 0.5387    | 0.0136    | 0.0013    | 0.0001    | 0.0000    | -76.5884      |
| 2p         | 0.4672    | 0.0269    | 0.0043    | 0.0004    | 0.0001    | -69.7769      |
| 3s         | 0.0993    | 0.0025    | 0.0002    | 0.0000    | 0.0000    | -11.8088      |
| 3p         | 0.0464    | 0.0036    | 0.0006    | 0.0001    | 0.0000    | -9.3161       |
| 3d         | -0.0361   | -0.0021   | -0.0003   | -0.0000   | -0.0000   | -4.8056       |
| 4s         | 0.0094    | 0.0001    | -0.0000   | -0.0000   | -0.0000   | -1.4552       |
| 4p         | 0.0004    | 0.0002    | 0.0000    | 0.0000    | 0.0000    | -0.8431       |
| 5s         | 0.0003    | 0.0000    | -0.0000   | -0.0000   | -0.0000   | -0.1278       |
| $\Delta E$ | 6.1604440 | 0.3357622 | 0.0580049 | 0.0069431 | 0.0018894 | -3132.9486592 |

Table S70: Errors in positions of orbital density maxima in bohr for the Sr atom computed with PBE and the regularized potential with various values of  $a$ . The values obtained with the Coulomb potential of the point nucleus are shown in the last column.

| Energy | $a = 1.0$ | $a = 2.0$ | $a = 3.0$ | $a = 5.0$ | $a = 7.0$ | point nucleus |
|--------|-----------|-----------|-----------|-----------|-----------|---------------|
| 1s     | 0.000146  | -0.000212 | -0.000002 | 0.000000  | 0.000000  | 0.026557      |
| 2s     | 0.000867  | 0.000026  | 0.000003  | 0.000000  | 0.000000  | 0.149269      |
| 2p     | 0.000922  | 0.000052  | 0.000008  | 0.000001  | 0.000000  | 0.117842      |
| 3s     | 0.002371  | 0.000072  | 0.000008  | 0.000001  | 0.000000  | 0.446088      |
| 3p     | 0.001673  | 0.000115  | 0.000019  | 0.000002  | 0.000000  | 0.435234      |
| 3d     | -0.000498 | -0.000033 | -0.000005 | -0.000000 | -0.000000 | 0.376330      |
| 4s     | 0.005596  | 0.000148  | 0.000014  | 0.000001  | 0.000001  | 1.216066      |
| 4p     | 0.003281  | 0.000255  | 0.000044  | 0.000004  | 0.000001  | 1.335481      |
| 5s     | 0.013269  | 0.000162  | -0.000008 | -0.000002 | 0.000000  | 3.766503      |

Table S71: Errors in orbital energies in  $E_h$  for the Sr atom computed with TASKCC and the regularized potential with various values of  $a$ . The values obtained with the Coulomb potential of the point nucleus are shown in the last column. For comparison, the last row shows the errors in total energy  $\Delta E$  from the point nucleus value shown in the last column.

| Energy     | $a = 1.0$ | $a = 2.0$ | $a = 3.0$ | $a = 5.0$ | $a = 7.0$ | point nucleus |
|------------|-----------|-----------|-----------|-----------|-----------|---------------|
| 1s         | -0.8641   | -0.0560   | -0.0080   | -0.0005   | -0.0001   | -575.1713     |
| 2s         | 0.5392    | 0.0132    | 0.0011    | 0.0000    | 0.0000    | -77.3286      |
| 2p         | 0.4682    | 0.0273    | 0.0044    | 0.0004    | 0.0001    | -70.4141      |
| 3s         | 0.1008    | 0.0025    | 0.0002    | 0.0000    | -0.0000   | -12.1573      |
| 3p         | 0.0470    | 0.0036    | 0.0006    | 0.0001    | 0.0000    | -9.6038       |
| 3d         | -0.0369   | -0.0021   | -0.0003   | -0.0000   | -0.0000   | -4.9646       |
| 4s         | 0.0099    | 0.0001    | -0.0000   | -0.0000   | -0.0000   | -1.5654       |
| 4p         | 0.0004    | 0.0002    | 0.0000    | 0.0000    | 0.0000    | -0.9153       |
| 5s         | 0.0004    | 0.0000    | -0.0000   | -0.0000   | -0.0000   | -0.1337       |
| $\Delta E$ | 6.1073567 | 0.3170417 | 0.0497152 | 0.0045576 | 0.0009172 | -3132.4842944 |

Table S72: Errors in positions of orbital density maxima in bohr for the Sr atom computed with TASKCC and the regularized potential with various values of  $a$ . The values obtained with the Coulomb potential of the point nucleus are shown in the last column.

| Energy | $a = 1.0$ | $a = 2.0$ | $a = 3.0$ | $a = 5.0$ | $a = 7.0$ | point nucleus |
|--------|-----------|-----------|-----------|-----------|-----------|---------------|
| 1s     | 0.000144  | -0.000211 | -0.000002 | 0.000000  | 0.000000  | 0.026567      |
| 2s     | 0.000868  | 0.000025  | 0.000003  | 0.000000  | 0.000000  | 0.149357      |
| 2p     | 0.000922  | 0.000053  | 0.000008  | 0.000001  | 0.000000  | 0.117869      |
| 3s     | 0.002367  | 0.000070  | 0.000007  | 0.000000  | 0.000000  | 0.446475      |
| 3p     | 0.001665  | 0.000115  | 0.000019  | 0.000002  | 0.000000  | 0.435444      |
| 3d     | -0.000494 | -0.000033 | -0.000005 | -0.000001 | -0.000000 | 0.376866      |
| 4s     | 0.005672  | 0.000155  | 0.000014  | 0.000001  | 0.000000  | 1.220887      |
| 4p     | 0.003421  | 0.000263  | 0.000045  | 0.000004  | 0.000001  | 1.335444      |
| 5s     | 0.016730  | 0.000139  | -0.000029 | -0.000006 | -0.000002 | 4.065596      |

Table S73: Errors in orbital energies in  $E_h$  for the Cd atom computed with HF and the regularized potential with various values of  $a$ . The values obtained with the Coulomb potential of the point nucleus are shown in the last column. For comparison, the last row shows the errors in total energy  $\Delta E$  from the point nucleus value shown in the last column.

| Energy     | $a = 1.0$  | $a = 2.0$ | $a = 3.0$ | $a = 5.0$ | $a = 7.0$ | point nucleus |
|------------|------------|-----------|-----------|-----------|-----------|---------------|
| 1s         | -1.0584    | -0.0744   | -0.0120   | -0.0010   | -0.0002   | -955.3154     |
| 2s         | 1.0246     | 0.0270    | 0.0023    | 0.0001    | -0.0000   | -142.0068     |
| 2p         | 0.8653     | 0.0507    | 0.0082    | 0.0007    | 0.0001    | -132.0470     |
| 3s         | 0.2370     | 0.0067    | 0.0006    | 0.0000    | -0.0000   | -27.7086      |
| 3p         | 0.1209     | 0.0091    | 0.0016    | 0.0001    | 0.0000    | -23.5972      |
| 3d         | -0.0523    | -0.0032   | -0.0005   | -0.0000   | -0.0000   | -16.0720      |
| 4s         | 0.0449     | 0.0014    | 0.0001    | 0.0000    | 0.0000    | -4.4505       |
| 4p         | 0.0168     | 0.0015    | 0.0003    | 0.0000    | 0.0000    | -3.0535       |
| 4d         | -0.0082    | -0.0004   | -0.0001   | -0.0000   | -0.0000   | -0.7637       |
| 5s         | 0.0024     | 0.0001    | 0.0000    | 0.0000    | 0.0000    | -0.2649       |
| $\Delta E$ | 10.7672549 | 0.5446860 | 0.0823369 | 0.0071407 | 0.0013954 | -5465.1331425 |

Table S74: Errors in positions of orbital density maxima in bohr for the Cd atom computed with HF and the regularized potential with various values of  $a$ . The values obtained with the Coulomb potential of the point nucleus are shown in the last column.

| Energy | $a = 1.0$ | $a = 2.0$ | $a = 3.0$ | $a = 5.0$ | $a = 7.0$ | point nucleus |
|--------|-----------|-----------|-----------|-----------|-----------|---------------|
| 1s     | 0.000125  | -0.000168 | -0.000002 | -0.000000 | 0.000000  | 0.020993      |
| 2s     | 0.000712  | 0.000021  | 0.000002  | 0.000000  | 0.000000  | 0.116292      |
| 2p     | 0.000720  | 0.000041  | 0.000007  | 0.000001  | 0.000000  | 0.091332      |
| 3s     | 0.001788  | 0.000055  | 0.000006  | 0.000000  | 0.000000  | 0.334770      |
| 3p     | 0.001177  | 0.000082  | 0.000014  | 0.000001  | 0.000000  | 0.322031      |
| 3d     | -0.000199 | -0.000016 | -0.000003 | -0.000000 | 0.000000  | 0.266427      |
| 4s     | 0.003935  | 0.000121  | 0.000012  | 0.000000  | 0.000000  | 0.822684      |
| 4p     | 0.002421  | 0.000181  | 0.000031  | 0.000003  | 0.000001  | 0.859507      |
| 4d     | -0.001573 | -0.000101 | -0.000016 | -0.000001 | -0.000000 | 0.977260      |
| 5s     | 0.019640  | 0.000649  | 0.000069  | 0.000004  | 0.000001  | 2.583744      |

Table S75: Errors in orbital energies in  $E_h$  for the Cd atom computed with PW92 and the regularized potential with various values of  $a$ . The values obtained with the Coulomb potential of the point nucleus are shown in the last column. For comparison, the last row shows the errors in total energy  $\Delta E$  from the point nucleus value shown in the last column.

| Energy     | $a = 1.0$  | $a = 2.0$ | $a = 3.0$ | $a = 5.0$ | $a = 7.0$ | point nucleus |
|------------|------------|-----------|-----------|-----------|-----------|---------------|
| 1s         | -1.2187    | -0.0806   | -0.0118   | -0.0008   | -0.0001   | -941.4768     |
| 2s         | 0.9873     | 0.0265    | 0.0024    | 0.0001    | 0.0000    | -136.8325     |
| 2p         | 0.8498     | 0.0497    | 0.0080    | 0.0007    | 0.0001    | -127.6351     |
| 3s         | 0.2206     | 0.0063    | 0.0006    | 0.0000    | 0.0000    | -25.3798      |
| 3p         | 0.1125     | 0.0085    | 0.0015    | 0.0001    | 0.0000    | -21.6374      |
| 3d         | -0.0498    | -0.0030   | -0.0005   | -0.0000   | -0.0000   | -14.6851      |
| 4s         | 0.0434     | 0.0013    | 0.0001    | 0.0000    | 0.0000    | -3.5959       |
| 4p         | 0.0171     | 0.0015    | 0.0003    | 0.0000    | 0.0000    | -2.3951       |
| 4d         | -0.0062    | -0.0003   | -0.0000   | -0.0000   | -0.0000   | -0.4704       |
| 5s         | 0.0022     | 0.0001    | 0.0000    | 0.0000    | 0.0000    | -0.2042       |
| $\Delta E$ | 10.7482876 | 0.5574430 | 0.0866174 | 0.0078343 | 0.0015726 | -5462.3711357 |

Table S76: Errors in positions of orbital density maxima in bohr for the Cd atom computed with PW92 and the regularized potential with various values of  $a$ . The values obtained with the Coulomb potential of the point nucleus are shown in the last column.

| Energy | $a = 1.0$ | $a = 2.0$ | $a = 3.0$ | $a = 5.0$ | $a = 7.0$ | point nucleus |
|--------|-----------|-----------|-----------|-----------|-----------|---------------|
| 1s     | 0.000121  | -0.000168 | -0.000002 | -0.000000 | 0.000000  | 0.021009      |
| 2s     | 0.000703  | 0.000021  | 0.000002  | 0.000000  | 0.000000  | 0.116595      |
| 2p     | 0.000718  | 0.000041  | 0.000007  | 0.000001  | 0.000000  | 0.091287      |
| 3s     | 0.001800  | 0.000055  | 0.000006  | 0.000000  | 0.000000  | 0.336464      |
| 3p     | 0.001180  | 0.000083  | 0.000014  | 0.000001  | 0.000000  | 0.322771      |
| 3d     | -0.000195 | -0.000016 | -0.000003 | -0.000000 | -0.000000 | 0.265871      |
| 4s     | 0.004024  | 0.000119  | 0.000011  | 0.000000  | 0.000000  | 0.821070      |
| 4p     | 0.002439  | 0.000188  | 0.000032  | 0.000003  | 0.000001  | 0.855640      |
| 4d     | -0.001837 | -0.000119 | -0.000019 | -0.000002 | -0.000000 | 0.974533      |
| 5s     | 0.016894  | 0.000554  | 0.000060  | 0.000004  | 0.000001  | 2.426584      |

Table S77: Errors in orbital energies in  $E_h$  for the Cd atom computed with PBE and the regularized potential with various values of  $a$ . The values obtained with the Coulomb potential of the point nucleus are shown in the last column. For comparison, the last row shows the errors in total energy  $\Delta E$  from the point nucleus value shown in the last column.

| Energy     | $a = 1.0$  | $a = 2.0$ | $a = 3.0$ | $a = 5.0$ | $a = 7.0$ | point nucleus |
|------------|------------|-----------|-----------|-----------|-----------|---------------|
| $1s$       | -1.1768    | -0.0711   | -0.0083   | 0.0001    | 0.0003    | -942.5807     |
| $2s$       | 0.9963     | 0.0277    | 0.0028    | 0.0002    | 0.0000    | -136.9562     |
| $2p$       | 0.8491     | 0.0496    | 0.0080    | 0.0007    | 0.0001    | -127.6759     |
| $3s$       | 0.2232     | 0.0066    | 0.0007    | 0.0000    | 0.0000    | -25.4181      |
| $3p$       | 0.1127     | 0.0085    | 0.0015    | 0.0001    | 0.0000    | -21.6485      |
| $3d$       | -0.0502    | -0.0030   | -0.0005   | -0.0000   | -0.0000   | -14.6734      |
| $4s$       | 0.0433     | 0.0014    | 0.0001    | 0.0000    | 0.0000    | -3.6013       |
| $4p$       | 0.0169     | 0.0015    | 0.0003    | 0.0000    | 0.0000    | -2.3951       |
| $4d$       | -0.0062    | -0.0003   | -0.0000   | -0.0000   | -0.0000   | -0.4645       |
| $5s$       | 0.0021     | 0.0001    | 0.0000    | 0.0000    | 0.0000    | -0.1940       |
| $\Delta E$ | 10.9260825 | 0.5933252 | 0.0994183 | 0.0110927 | 0.0028529 | -5467.0515829 |

Table S78: Errors in positions of orbital density maxima in bohr for the Cd atom computed with PBE and the regularized potential with various values of  $a$ . The values obtained with the Coulomb potential of the point nucleus are shown in the last column.

| Energy | $a = 1.0$ | $a = 2.0$ | $a = 3.0$ | $a = 5.0$ | $a = 7.0$ | point nucleus |
|--------|-----------|-----------|-----------|-----------|-----------|---------------|
| $1s$   | 0.000126  | -0.000168 | -0.000002 | 0.000000  | 0.000000  | 0.020988      |
| $2s$   | 0.000709  | 0.000022  | 0.000002  | 0.000000  | 0.000000  | 0.116470      |
| $2p$   | 0.000719  | 0.000041  | 0.000007  | 0.000001  | 0.000000  | 0.091278      |
| $3s$   | 0.001805  | 0.000057  | 0.000006  | 0.000000  | 0.000000  | 0.336003      |
| $3p$   | 0.001177  | 0.000083  | 0.000014  | 0.000001  | 0.000000  | 0.322543      |
| $3d$   | -0.000195 | -0.000016 | -0.000003 | -0.000000 | 0.000000  | 0.266251      |
| $4s$   | 0.004027  | 0.000123  | 0.000013  | 0.000001  | 0.000000  | 0.821914      |
| $4p$   | 0.002432  | 0.000186  | 0.000032  | 0.000003  | 0.000001  | 0.856916      |
| $4d$   | -0.001741 | -0.000114 | -0.000018 | -0.000002 | -0.000000 | 0.975060      |
| $5s$   | 0.017794  | 0.000603  | 0.000069  | 0.000005  | 0.000001  | 2.443583      |

Table S79: Errors in orbital energies in  $E_h$  for the Cd atom computed with TASKCC and the regularized potential with various values of  $a$ . The values obtained with the Coulomb potential of the point nucleus are shown in the last column. For comparison, the last row shows the errors in total energy  $\Delta E$  from the point nucleus value shown in the last column.

| Energy     | $a = 1.0$  | $a = 2.0$ | $a = 3.0$ | $a = 5.0$ | $a = 7.0$ | point nucleus |
|------------|------------|-----------|-----------|-----------|-----------|---------------|
| $1s$       | -1.1327    | -0.0743   | -0.0107   | -0.0007   | -0.0001   | -944.3845     |
| $2s$       | 0.9966     | 0.0272    | 0.0025    | 0.0001    | 0.0000    | -137.9301     |
| $2p$       | 0.8492     | 0.0500    | 0.0081    | 0.0007    | 0.0001    | -128.5216     |
| $3s$       | 0.2253     | 0.0066    | 0.0006    | 0.0000    | 0.0000    | -25.8327      |
| $3p$       | 0.1133     | 0.0087    | 0.0015    | 0.0001    | 0.0000    | -21.9992      |
| $3d$       | -0.0516    | -0.0031   | -0.0005   | -0.0000   | -0.0000   | -14.8893      |
| $4s$       | 0.0430     | 0.0013    | 0.0001    | 0.0000    | 0.0000    | -3.7500       |
| $4p$       | 0.0164     | 0.0014    | 0.0003    | 0.0000    | 0.0000    | -2.5068       |
| $4d$       | -0.0069    | -0.0003   | -0.0000   | -0.0000   | -0.0000   | -0.4941       |
| $5s$       | 0.0026     | 0.0001    | 0.0000    | 0.0000    | 0.0000    | -0.2116       |
| $\Delta E$ | 10.8525107 | 0.5690307 | 0.0886970 | 0.0080088 | 0.0015962 | -5466.3121236 |

Table S80: Errors in positions of orbital density maxima in bohr for the Cd atom computed with TASKCC and the regularized potential with various values of  $a$ . The values obtained with the Coulomb potential of the point nucleus are shown in the last column.

| Energy | $a = 1.0$ | $a = 2.0$ | $a = 3.0$ | $a = 5.0$ | $a = 7.0$ | point nucleus |
|--------|-----------|-----------|-----------|-----------|-----------|---------------|
| $1s$   | 0.000125  | -0.000168 | -0.000002 | 0.000000  | 0.000000  | 0.020995      |
| $2s$   | 0.000709  | 0.000022  | 0.000002  | 0.000000  | 0.000000  | 0.116536      |
| $2p$   | 0.000718  | 0.000041  | 0.000007  | 0.000001  | 0.000000  | 0.091305      |
| $3s$   | 0.001801  | 0.000056  | 0.000006  | 0.000000  | 0.000000  | 0.336151      |
| $3p$   | 0.001172  | 0.000083  | 0.000014  | 0.000001  | 0.000000  | 0.322573      |
| $3d$   | -0.000194 | -0.000016 | -0.000003 | -0.000000 | -0.000000 | 0.266346      |
| $4s$   | 0.004011  | 0.000122  | 0.000012  | 0.000001  | 0.000000  | 0.824853      |
| $4p$   | 0.002430  | 0.000186  | 0.000032  | 0.000003  | 0.000001  | 0.859683      |
| $4d$   | -0.001637 | -0.000108 | -0.000017 | -0.000001 | -0.000000 | 0.975390      |
| $5s$   | 0.022381  | 0.000765  | 0.000086  | 0.000005  | 0.000001  | 2.449810      |

Table S81: Errors in orbital energies in  $E_h$  for the Xe atom computed with HF and the regularized potential with various values of  $a$ . The values obtained with the Coulomb potential of the point nucleus are shown in the last column. For comparison, the last row shows the errors in total energy  $\Delta E$  from the point nucleus value shown in the last column.

| Energy     | $a = 1.0$  | $a = 2.0$ | $a = 3.0$ | $a = 5.0$ | $a = 7.0$ | point nucleus |
|------------|------------|-----------|-----------|-----------|-----------|---------------|
| $1s$       | -1.2223    | -0.0864   | -0.0140   | -0.0012   | -0.0002   | -1224.3978    |
| $2s$       | 1.3612     | 0.0369    | 0.0033    | 0.0001    | 0.0000    | -189.3401     |
| $2p$       | 1.1398     | 0.0670    | 0.0108    | 0.0010    | 0.0002    | -177.7824     |
| $3s$       | 0.3273     | 0.0093    | 0.0008    | 0.0000    | -0.0000   | -40.1757      |
| $3p$       | 0.1630     | 0.0124    | 0.0021    | 0.0002    | 0.0000    | -35.2217      |
| $3d$       | -0.0715    | -0.0046   | -0.0007   | -0.0001   | -0.0000   | -26.1189      |
| $4s$       | 0.0667     | 0.0018    | 0.0001    | 0.0000    | -0.0000   | -7.8563       |
| $4p$       | 0.0229     | 0.0020    | 0.0004    | 0.0000    | 0.0000    | -6.0083       |
| $4d$       | -0.0189    | -0.0012   | -0.0002   | -0.0000   | -0.0000   | -2.7779       |
| $5s$       | 0.0071     | 0.0001    | -0.0000   | -0.0000   | -0.0000   | -0.9444       |
| $5p$       | 0.0003     | 0.0001    | 0.0000    | 0.0000    | 0.0000    | -0.4573       |
| $\Delta E$ | 14.3548617 | 0.7337275 | 0.1112116 | 0.0096472 | 0.0018832 | -7232.1383639 |

Table S82: Errors in positions of orbital density maxima in bohr for the Xe atom computed with HF and the regularized potential with various values of  $a$ . The values obtained with the Coulomb potential of the point nucleus are shown in the last column.

| Energy | $a = 1.0$ | $a = 2.0$ | $a = 3.0$ | $a = 5.0$ | $a = 7.0$ | point nucleus |
|--------|-----------|-----------|-----------|-----------|-----------|---------------|
| $1s$   | 0.000115  | -0.000149 | -0.000002 | -0.000000 | 0.000000  | 0.018646      |
| $2s$   | 0.000640  | 0.000019  | 0.000002  | 0.000000  | 0.000000  | 0.102751      |
| $2p$   | 0.000635  | 0.000037  | 0.000006  | 0.000001  | 0.000000  | 0.080437      |
| $3s$   | 0.001573  | 0.000050  | 0.000005  | 0.000000  | 0.000000  | 0.291303      |
| $3p$   | 0.001002  | 0.000071  | 0.000012  | 0.000001  | 0.000000  | 0.278426      |
| $3d$   | -0.000121 | -0.000011 | -0.000002 | -0.000000 | -0.000000 | 0.226670      |
| $4s$   | 0.003203  | 0.000101  | 0.000010  | 0.000000  | 0.000000  | 0.687112      |
| $4p$   | 0.001838  | 0.000140  | 0.000024  | 0.000002  | 0.000000  | 0.704892      |
| $4d$   | -0.000809 | -0.000056 | -0.000009 | -0.000001 | -0.000000 | 0.746845      |
| $5s$   | 0.008100  | 0.000233  | 0.000020  | 0.000000  | 0.000000  | 1.713121      |
| $5p$   | 0.004144  | 0.000349  | 0.000061  | 0.000006  | 0.000002  | 1.939680      |

Table S83: Errors in orbital energies in  $E_h$  for the Xe atom computed with PW92 and the regularized potential with various values of  $a$ . The values obtained with the Coulomb potential of the point nucleus are shown in the last column. For comparison, the last row shows the errors in total energy  $\Delta E$  from the point nucleus value shown in the last column.

| Energy     | $a = 1.0$  | $a = 2.0$ | $a = 3.0$ | $a = 5.0$ | $a = 7.0$ | point nucleus |
|------------|------------|-----------|-----------|-----------|-----------|---------------|
| 1s         | -1.4064    | -0.0937   | -0.0138   | -0.0010   | -0.0001   | -1208.6891    |
| 2s         | 1.3173     | 0.0362    | 0.0034    | 0.0001    | 0.0000    | -183.3275     |
| 2p         | 1.1219     | 0.0659    | 0.0106    | 0.0010    | 0.0002    | -172.5996     |
| 3s         | 0.3068     | 0.0088    | 0.0008    | 0.0000    | 0.0000    | -37.4153      |
| 3p         | 0.1525     | 0.0116    | 0.0020    | 0.0002    | 0.0000    | -32.8669      |
| 3d         | -0.0695    | -0.0045   | -0.0007   | -0.0001   | -0.0000   | -24.3781      |
| 4s         | 0.0630     | 0.0016    | 0.0001    | 0.0000    | -0.0000   | -6.6782       |
| 4p         | 0.0218     | 0.0019    | 0.0003    | 0.0000    | 0.0000    | -5.0636       |
| 4d         | -0.0175    | -0.0011   | -0.0002   | -0.0000   | -0.0000   | -2.2865       |
| 5s         | 0.0063     | 0.0000    | -0.0000   | -0.0000   | -0.0000   | -0.6720       |
| 5p         | 0.0000     | 0.0000    | 0.0000    | 0.0000    | 0.0000    | -0.3098       |
| $\Delta E$ | 14.3255451 | 0.7477595 | 0.1160029 | 0.0104290 | 0.0020834 | -7228.8341637 |

Table S84: Errors in positions of orbital density maxima in bohr for the Xe atom computed with PW92 and the regularized potential with various values of  $a$ . The values obtained with the Coulomb potential of the point nucleus are shown in the last column.

| Energy | $a = 1.0$ | $a = 2.0$ | $a = 3.0$ | $a = 5.0$ | $a = 7.0$ | point nucleus |
|--------|-----------|-----------|-----------|-----------|-----------|---------------|
| 1s     | 0.000112  | -0.000149 | -0.000002 | -0.000000 | 0.000000  | 0.018658      |
| 2s     | 0.000633  | 0.000019  | 0.000002  | 0.000000  | 0.000000  | 0.102982      |
| 2p     | 0.000634  | 0.000037  | 0.000006  | 0.000001  | 0.000000  | 0.080402      |
| 3s     | 0.001578  | 0.000050  | 0.000005  | 0.000000  | 0.000000  | 0.292694      |
| 3p     | 0.001002  | 0.000071  | 0.000012  | 0.000001  | 0.000000  | 0.279112      |
| 3d     | -0.000119 | -0.000011 | -0.000002 | -0.000000 | 0.000000  | 0.226503      |
| 4s     | 0.003310  | 0.000101  | 0.000010  | 0.000000  | 0.000000  | 0.688477      |
| 4p     | 0.001874  | 0.000147  | 0.000025  | 0.000002  | 0.000001  | 0.705072      |
| 4d     | -0.000911 | -0.000063 | -0.000010 | -0.000001 | -0.000000 | 0.745465      |
| 5s     | 0.008332  | 0.000219  | 0.000017  | 0.000000  | 0.000000  | 1.686624      |
| 5p     | 0.003849  | 0.000358  | 0.000064  | 0.000006  | 0.000001  | 1.924671      |

Table S85: Errors in orbital energies in  $E_h$  for the Xe atom computed with PBE and the regularized potential with various values of  $a$ . The values obtained with the Coulomb potential of the point nucleus are shown in the last column. For comparison, the last row shows the errors in total energy  $\Delta E$  from the point nucleus value shown in the last column.

| Energy     | $a = 1.0$  | $a = 2.0$ | $a = 3.0$ | $a = 5.0$ | $a = 7.0$ | point nucleus |
|------------|------------|-----------|-----------|-----------|-----------|---------------|
| 1s         | -1.3583    | -0.0828   | -0.0098   | 0.0001    | 0.0003    | -1209.9445    |
| 2s         | 1.3279     | 0.0376    | 0.0038    | 0.0002    | 0.0001    | -183.4753     |
| 2p         | 1.1214     | 0.0658    | 0.0106    | 0.0010    | 0.0002    | -172.6537     |
| 3s         | 0.3101     | 0.0091    | 0.0009    | 0.0000    | 0.0000    | -37.4570      |
| 3p         | 0.1528     | 0.0116    | 0.0020    | 0.0002    | 0.0000    | -32.8802      |
| 3d         | -0.0699    | -0.0045   | -0.0007   | -0.0001   | -0.0000   | -24.3707      |
| 4s         | 0.0633     | 0.0017    | 0.0001    | 0.0000    | 0.0000    | -6.6979       |
| 4p         | 0.0217     | 0.0019    | 0.0003    | 0.0000    | 0.0000    | -5.0731       |
| 4d         | -0.0175    | -0.0011   | -0.0002   | -0.0000   | -0.0000   | -2.2840       |
| 5s         | 0.0062     | 0.0001    | -0.0000   | -0.0000   | -0.0000   | -0.6646       |
| 5p         | -0.0000    | 0.0000    | 0.0000    | 0.0000    | 0.0000    | -0.3046       |
| $\Delta E$ | 14.5286158 | 0.7886246 | 0.1305652 | 0.0141333 | 0.0035386 | -7234.2332120 |

Table S86: Errors in positions of orbital density maxima in bohr for the Xe atom computed with PBE and the regularized potential with various values of  $a$ . The values obtained with the Coulomb potential of the point nucleus are shown in the last column.

| Energy | $a = 1.0$ | $a = 2.0$ | $a = 3.0$ | $a = 5.0$ | $a = 7.0$ | point nucleus |
|--------|-----------|-----------|-----------|-----------|-----------|---------------|
| 1s     | 0.000116  | -0.000150 | -0.000002 | 0.000000  | 0.000000  | 0.018643      |
| 2s     | 0.000638  | 0.000020  | 0.000002  | 0.000000  | 0.000000  | 0.102887      |
| 2p     | 0.000634  | 0.000037  | 0.000006  | 0.000001  | 0.000000  | 0.080394      |
| 3s     | 0.001582  | 0.000051  | 0.000006  | 0.000000  | 0.000000  | 0.292305      |
| 3p     | 0.001000  | 0.000071  | 0.000012  | 0.000001  | 0.000000  | 0.278896      |
| 3d     | -0.000119 | -0.000011 | -0.000002 | -0.000000 | 0.000000  | 0.226728      |
| 4s     | 0.003302  | 0.000104  | 0.000011  | 0.000001  | 0.000000  | 0.688525      |
| 4p     | 0.001864  | 0.000145  | 0.000025  | 0.000002  | 0.000000  | 0.705356      |
| 4d     | -0.000868 | -0.000061 | -0.000010 | -0.000001 | -0.000000 | 0.745762      |
| 5s     | 0.008527  | 0.000236  | 0.000021  | 0.000001  | 0.000000  | 1.696320      |
| 5p     | 0.003968  | 0.000359  | 0.000063  | 0.000006  | 0.000001  | 1.934559      |



Table S87: Errors in orbital energies in  $E_h$  for the Xe atom computed with TASKCC and the regularized potential with various values of  $a$ . The values obtained with the Coulomb potential of the point nucleus are shown in the last column. For comparison, the last row shows the errors in total energy  $\Delta E$  from the point nucleus value shown in the last column.

| Energy     | $a = 1.0$  | $a = 2.0$ | $a = 3.0$ | $a = 5.0$ | $a = 7.0$ | point nucleus |
|------------|------------|-----------|-----------|-----------|-----------|---------------|
| 1s         | -1.3075    | -0.0864   | -0.0126   | -0.0008   | -0.0001   | -1212.0214    |
| 2s         | 1.3285     | 0.0370    | 0.0035    | 0.0001    | 0.0000    | -184.6493     |
| 2p         | 1.1213     | 0.0662    | 0.0107    | 0.0010    | 0.0002    | -173.6861     |
| 3s         | 0.3128     | 0.0090    | 0.0008    | 0.0000    | 0.0000    | -37.9716      |
| 3p         | 0.1536     | 0.0118    | 0.0020    | 0.0002    | 0.0000    | -33.3301      |
| 3d         | -0.0712    | -0.0046   | -0.0007   | -0.0001   | -0.0000   | -24.6824      |
| 4s         | 0.0637     | 0.0017    | 0.0001    | 0.0000    | -0.0000   | -6.9179       |
| 4p         | 0.0217     | 0.0019    | 0.0003    | 0.0000    | 0.0000    | -5.2477       |
| 4d         | -0.0178    | -0.0011   | -0.0002   | -0.0000   | -0.0000   | -2.3639       |
| 5s         | 0.0066     | 0.0001    | -0.0000   | -0.0000   | -0.0000   | -0.7190       |
| 5p         | -0.0000    | 0.0000    | 0.0000    | 0.0000    | 0.0000    | -0.3306       |
| $\Delta E$ | 14.4457645 | 0.7612456 | 0.1184265 | 0.0106325 | 0.0021111 | -7233.3416395 |

Table S88: Errors in positions of orbital density maxima in bohr for the Xe atom computed with TASKCC and the regularized potential with various values of  $a$ . The values obtained with the Coulomb potential of the point nucleus are shown in the last column.

| Energy | $a = 1.0$ | $a = 2.0$ | $a = 3.0$ | $a = 5.0$ | $a = 7.0$ | point nucleus |
|--------|-----------|-----------|-----------|-----------|-----------|---------------|
| 1s     | 0.000115  | -0.000150 | -0.000002 | -0.000000 | 0.000000  | 0.018648      |
| 2s     | 0.000638  | 0.000020  | 0.000002  | 0.000000  | 0.000000  | 0.102941      |
| 2p     | 0.000634  | 0.000037  | 0.000006  | 0.000001  | 0.000000  | 0.080418      |
| 3s     | 0.001579  | 0.000050  | 0.000005  | 0.000000  | 0.000000  | 0.292393      |
| 3p     | 0.000996  | 0.000071  | 0.000012  | 0.000001  | 0.000000  | 0.278905      |
| 3d     | -0.000118 | -0.000011 | -0.000002 | -0.000000 | 0.000000  | 0.226757      |
| 4s     | 0.003284  | 0.000102  | 0.000010  | 0.000000  | 0.000000  | 0.689832      |
| 4p     | 0.001849  | 0.000145  | 0.000025  | 0.000002  | 0.000001  | 0.706492      |
| 4d     | -0.000837 | -0.000059 | -0.000009 | -0.000001 | -0.000000 | 0.746263      |
| 5s     | 0.008732  | 0.000256  | 0.000024  | 0.000001  | 0.000000  | 1.709528      |
| 5p     | 0.004292  | 0.000377  | 0.000067  | 0.000007  | 0.000002  | 1.937097      |
